# Supplementary material for: ASSANet: An Anisotropic Separable Set Abstraction for Efficient Point Cloud Representation Learning
Source: arXiv:2110.10538 source file (2021-10-24)
Supplement: Supplementary file 1 [file supplement.tex]

\clearpage
\title{ASSANet: An Anisotropic Separable Set Abstraction \\ for Efficient Point Cloud Representation Learning \\
--Supplementary Material--
}

% The \author macro works with any number of authors. There are two commands
% used to separate the names and addresses of multiple authors: \And and \AND.
%
% Using \And between authors leaves it to LaTeX to determine where to break the
% lines. Using \AND forces a line break at that point. So, if LaTeX puts 3 of 4
% authors names on the first line, and the last on the second line, try using
% \AND instead of \And before the third author name.
\author{%
Guocheng Qian 
% KAUST\\
% \texttt{guocheng.qian@kaust.edu.sa} \\
\And
Hasan Abed Al Kader Hammoud 
% KAUST\\
% \texttt{guocheng.qian@kaust.edu.sa} \\
\And Guohao Li 
% KAUST\\
% \texttt{guocheng.qian@kaust.edu.sa} \\
\And Ali Thabet 
% KAUST\\
% \texttt{guocheng.qian@kaust.edu.sa} \\
\AND Bernard Ghanem \\ 
King Abdullah University of Science and Technology (KAUST)\\
\texttt{\{guocheng.qian, hasanabedalkader.hammoud, bernard.ghanem\}@kaust.edu.sa} \\
\url{https://github.com/guochengqian/ASSANet}
}

\maketitle

\setcounter{section}{0}

In this supplementary material, we provide a detailed analysis of the proposed Set Abstraction (SA) variants.

\section{More about SA Variants}
\subsection{Equivalence between PreConv SA and vanilla SA}
Our proposed PreConv SA is formulated in \eqnLabel \ref{eqn:preconv_sa}.
\begin{equation}\label{eqn:preconv_sa}
\begin{split}
\mathbf{f}_i^{\prime} & = \operatorname{MLPs}\left(\mathbf{f}_i^l\right)\\
\mathbf{f}_i^{l+1} &=\mathcal{R}\left(\left\{\mathbf{f}_j^{\prime}|j\in \mathcal{N}(i)\right\}\right),
\end{split}
\end{equation}

Here, we show that the proposed PreConv SA is equivalent to the vanilla SA when edge information is not used. In this case, the vanilla SA is formulated as follows:
\begin{equation}\label{eqn:reduced_sa}
\mathbf{f}_i^{l+1} =\mathcal{R}\left(\left\{\operatorname{MLPs}\left( \mathbf{f}_j^l\right)|j\in \mathcal{N}(i)\right\}\right),
\end{equation}

Since (1) the neighborhood querying function $\mathcal{N}(i)$ is independent on the point features, and (2) the MLPs is a \textbf{shared} point-wise function processed on each neighbor features,  \eqnLabel \ref{eqn:preconv_sa} is equivalent to \eqnLabel \ref{eqn:reduced_sa}.

\subsection{Pseudocode of ASSA}
We provide the pseudocode of the proposed ASSA module in \algLabel \ref{alg:code}. 
% \begin{wrapfigure}{r}{0.5\textwidth}
% \begin{minipage}{0.5\textwidth}
\begin{algorithm}[H]
\caption{Pseudocode of ASSA in a PyTorch-like style.}
\label{alg:code}
% \algcomment{\fontsize{7.2pt}{0em}\selectfont \texttt{*}: element wise multiplication.
%\vspace{-1.em}
% }
\definecolor{codeblue}{rgb}{0.25,0.5,0.5}
\lstset{
  backgroundcolor=\color{white},
  basicstyle=\fontsize{7.2pt}{7.2pt}\ttfamily\selectfont,
  columns=fullflexible,
  breaklines=true,
  captionpos=b,
  commentstyle=\fontsize{7.2pt}{7.2pt}\color{codeblue},
  keywordstyle=\fontsize{7.2pt}{7.2pt},
%  frame=tb,
}
\begin{lstlisting}[language=python]
# f: input features with shape: (B,C,N)
# p_q, p_s: (x,y,z) position for query and support 
# shortcut: nn.Linear(ceil(C/3), C)

# conduct MLPs on input point features
f = ReLU(MLP(f) + f) # (B,ceil(C/3),N)

# query the neighborhood features f_N (B,ceil(C/3),N,K)
# and the normalized relative position d_p (B,3,N,K)
f_N, d_p = Group(p_q, p_s, f) 

# repeat f_N to size (B,3,ceil(C/3),N,K)
# f_N is then element-wise weighted by d_p
f_N = f_N.expand(3, dim=1) * d_p
f_N = f_N.view(B, C, N, K)

# Reduction layer aggregates the neighborhood information 
# outputs f_aggr: (B,ceil(C/3)*3,N)
f_aggr = Reduction(f_N)

# MLPs on f_aggr and obtain f_out, output dimensions C
f_out = ReLU(MLP(f_aggr) + shortcut(f))
# return f_out with shape (B,C,N)
\end{lstlisting}
\end{algorithm}

\subsection{Difference of ASSA with previous work}
Our ASSA module can be viewed as a separable anisotropic graph convolution for point cloud learning. 
Inspired by the depthwise separable convolution used in MobileNet \cite{Howard2017MobileNetsEC}, we extend this separable idea to graph convolution. We only perform MLPs on point features directly to learn the channel correlation, and leverages the anisotropic reduction to aggregate the spatial correlation. Such anisotropic reduction was studied in adaptive weight-based point cloud learning methods like ParamConv \cite{wang2018deep}, RS-CNN \cite{Liu2019RelationShapeCN}, \etc. They used expensive computations to learn adaptive weights from the relative position or the local density. The recent paper by Liu \cite{Liu2020ACL} proposed PosPool, which simply leveraged the relative position vector $\mathbf{p}$ as the adaptive weights and outperformed previous methods. However, their method requires to divide the channels into three parts and scale the each part by $x, y, z$, respectively. This leads to performance degradation for two major reasons: first, the scaling is based on the heuristic grouping, and second, each scaling only sees one part of the feature instead of the whole information. On the contrary, our method does not conduct any grouping. The proposed Anisotropc Reduction scales the whole feature by three times, and then concatenate them together. We have shown the superiority of our Anisotropic Reduction and the ASSA module in terms of accuracy and speed in main paper Section 5.1.

\subsection{Illustration of PreConv SA and Separable SA}

\begin{figure}[!ht]

    \begin{subfigure}{1.3in}
        \includegraphics[height=60mm]{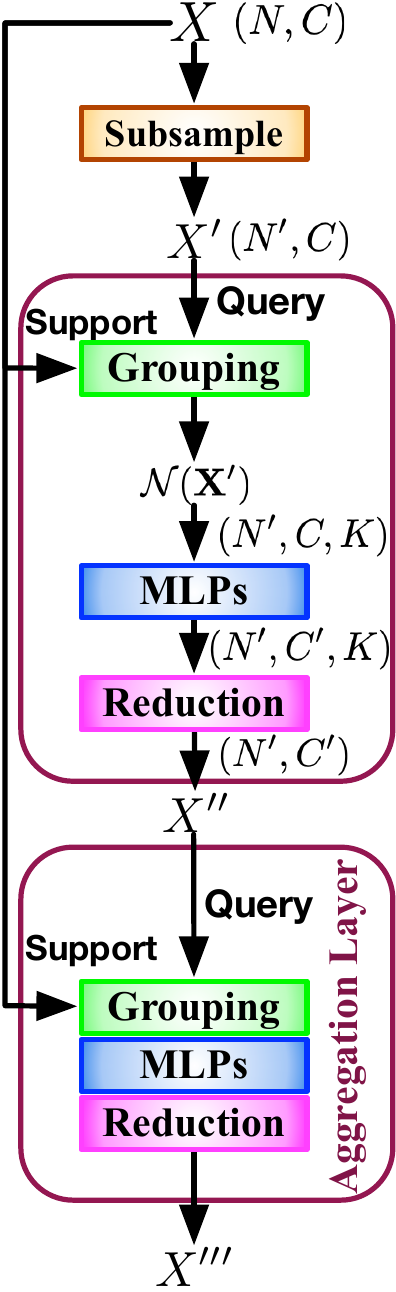}
        \caption{Vanilla SA}
        \label{fig:vanilla_sa}
    \end{subfigure}%
    \hfill
    \begin{subfigure}{1.3in}
        \includegraphics[height=60mm]{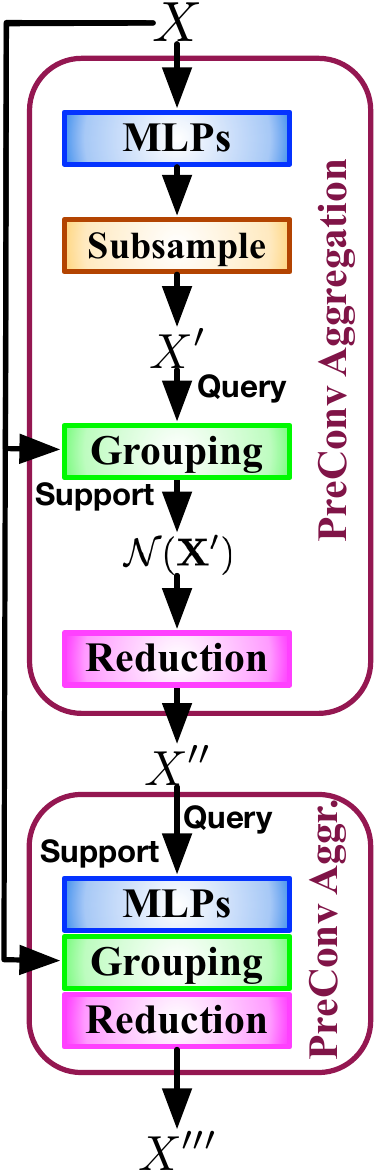}
        \caption{PreConv SA}
        \label{fig:vanilla_sa}
    \end{subfigure}%
    \hfill
    \begin{subfigure}{1.3in}
        \includegraphics[height=60mm]{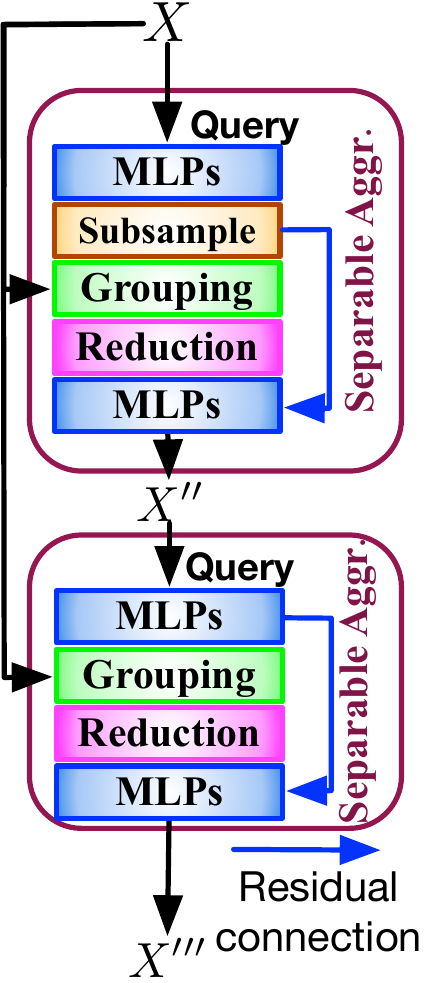}
        \caption{Separable SA}
        \label{fig:vanilla_sa}
    \end{subfigure}%
    \hfill
    \begin{subfigure}{1.3in}
        \includegraphics[height=60mm]{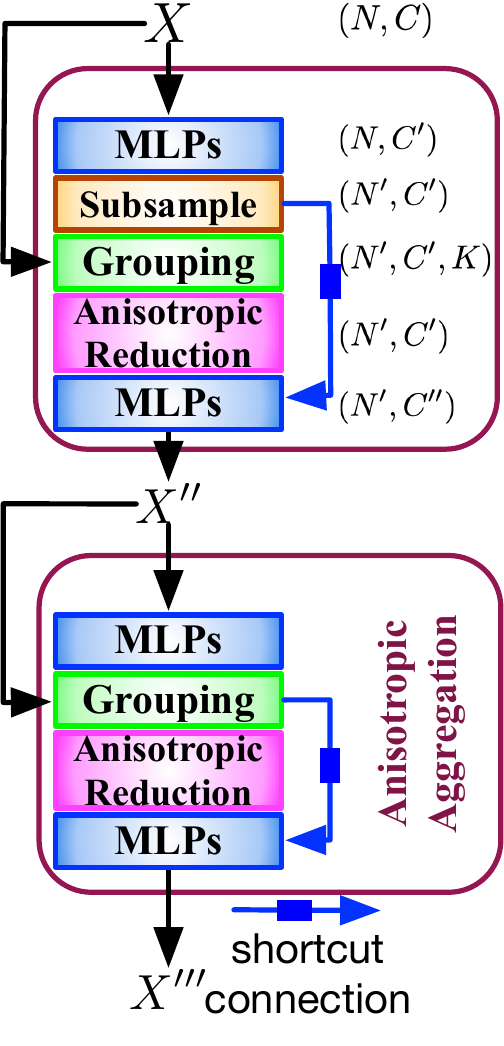}
        \caption{ASSA}
        \label{fig:vanilla_sa}
    \end{subfigure}%
    
\caption{
\textbf{Comparison of proposed variants of the Set Abstraction (SA) module and the Vanilla SA module.} (a) Vanilla SA \cite{Qi2017PointNetDH} applies MLPs on neighbor features. (b) The proposed PreConv SA applies MLPs on the point features directly. (c) Our Separable SA separates the MLPs to also process on the aggregated features from a local neighbors. (d) Our final ASSA module replaces the reduction layer in Separable SA with a new Anisotropic Reduction layer. 
$X, N, C, K$ are the input point cloud, the number of points, the number of input features, the number of neighbors. The shortcut layer in blue line is the residual connection with a linear mapping. The shortcut layer is the residual connection with a linear mapping. 
}
\end{figure}

\subsection{Latency analysis of ASSA compared with vanilla SA}
We show the latency decomposition of ASSA module only compared to vanilla SA module only. We show the cases using $4096$ points as input and $15,000$ points as input. In both case, our proposed ASSA module reduces the time consumed in computation part by $4\times$. 

\begin{figure}[!ht]
    \begin{subfigure}{0.45\textwidth}
        \includegraphics[height=40mm]{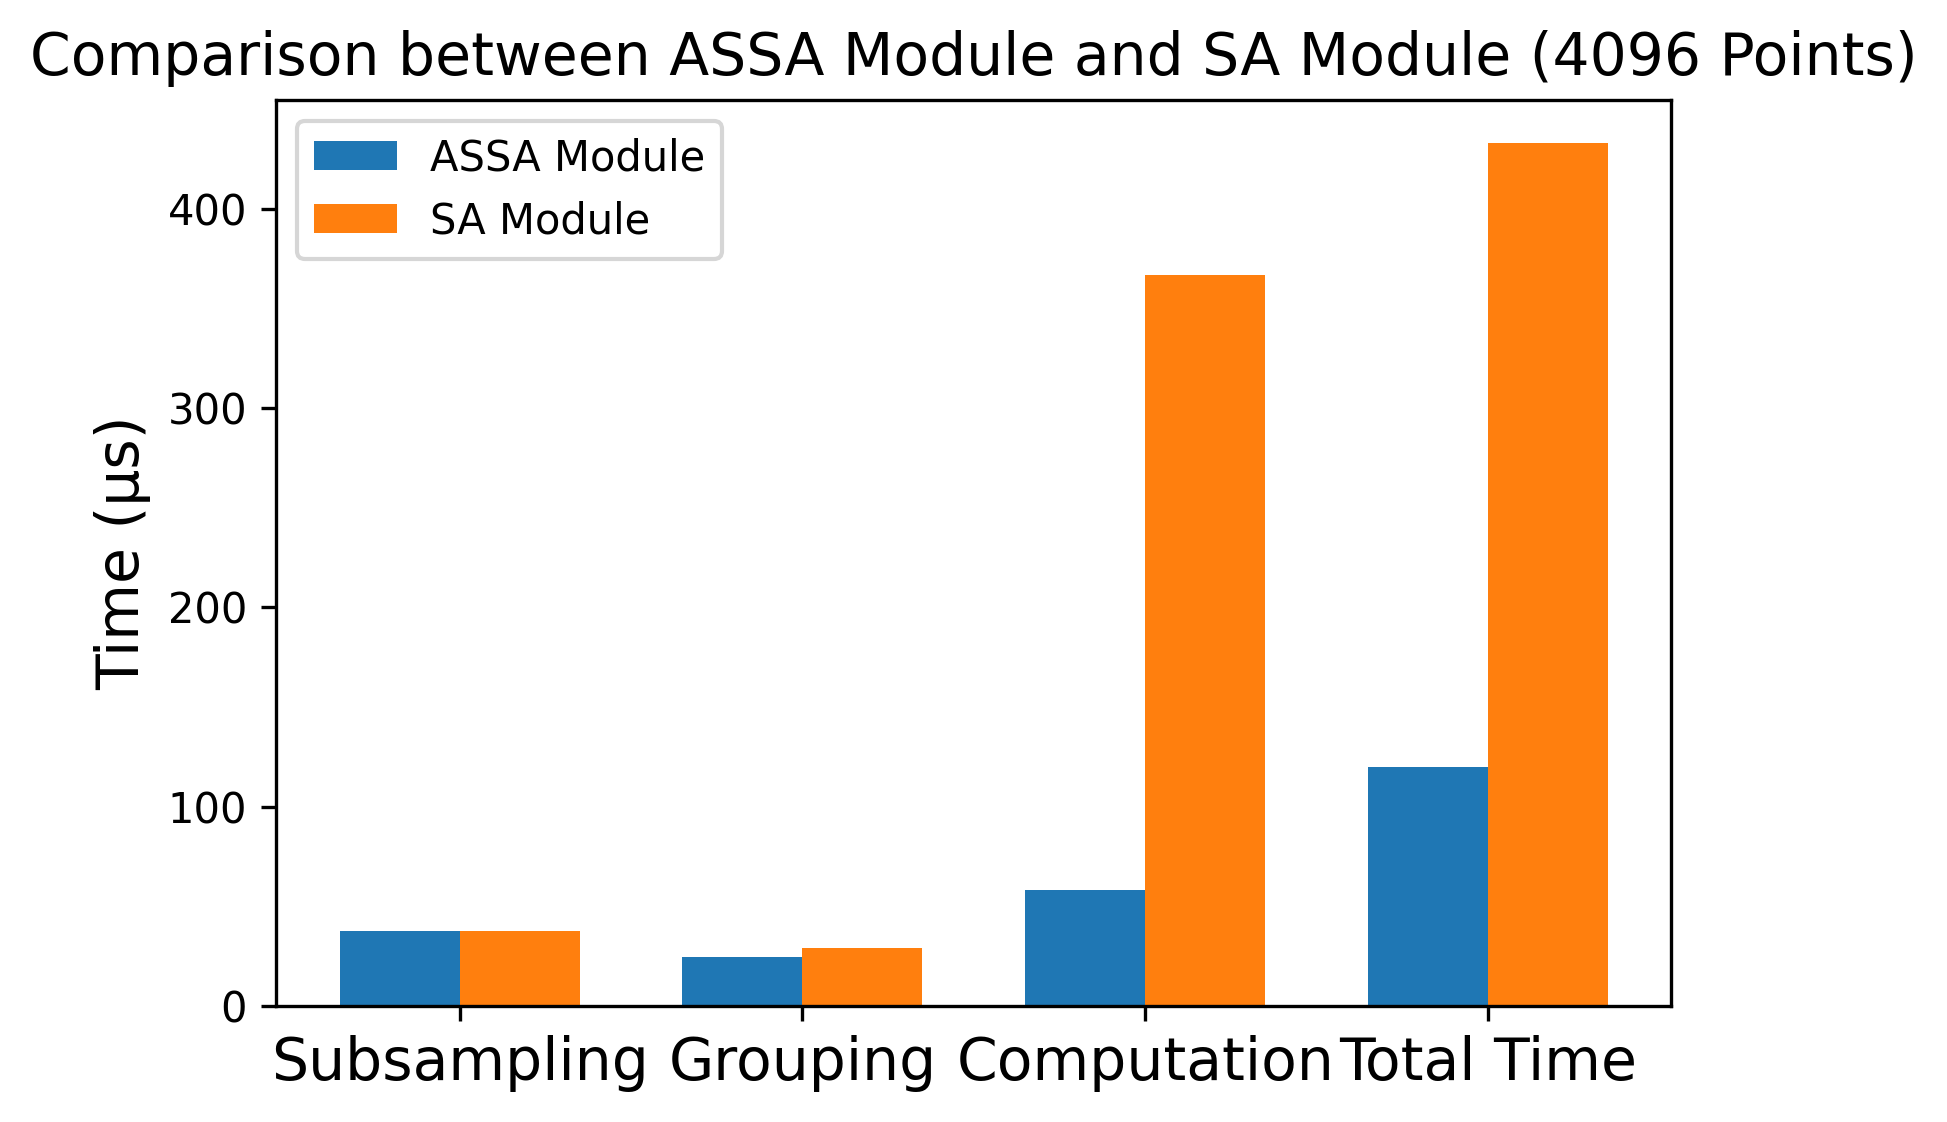}
        \caption{Latency decomposition (4096 points)}
        \label{fig:latency_4k}
    \end{subfigure}%
    \hfill
    \begin{subfigure}{0.45\textwidth}
        \includegraphics[height=40mm]{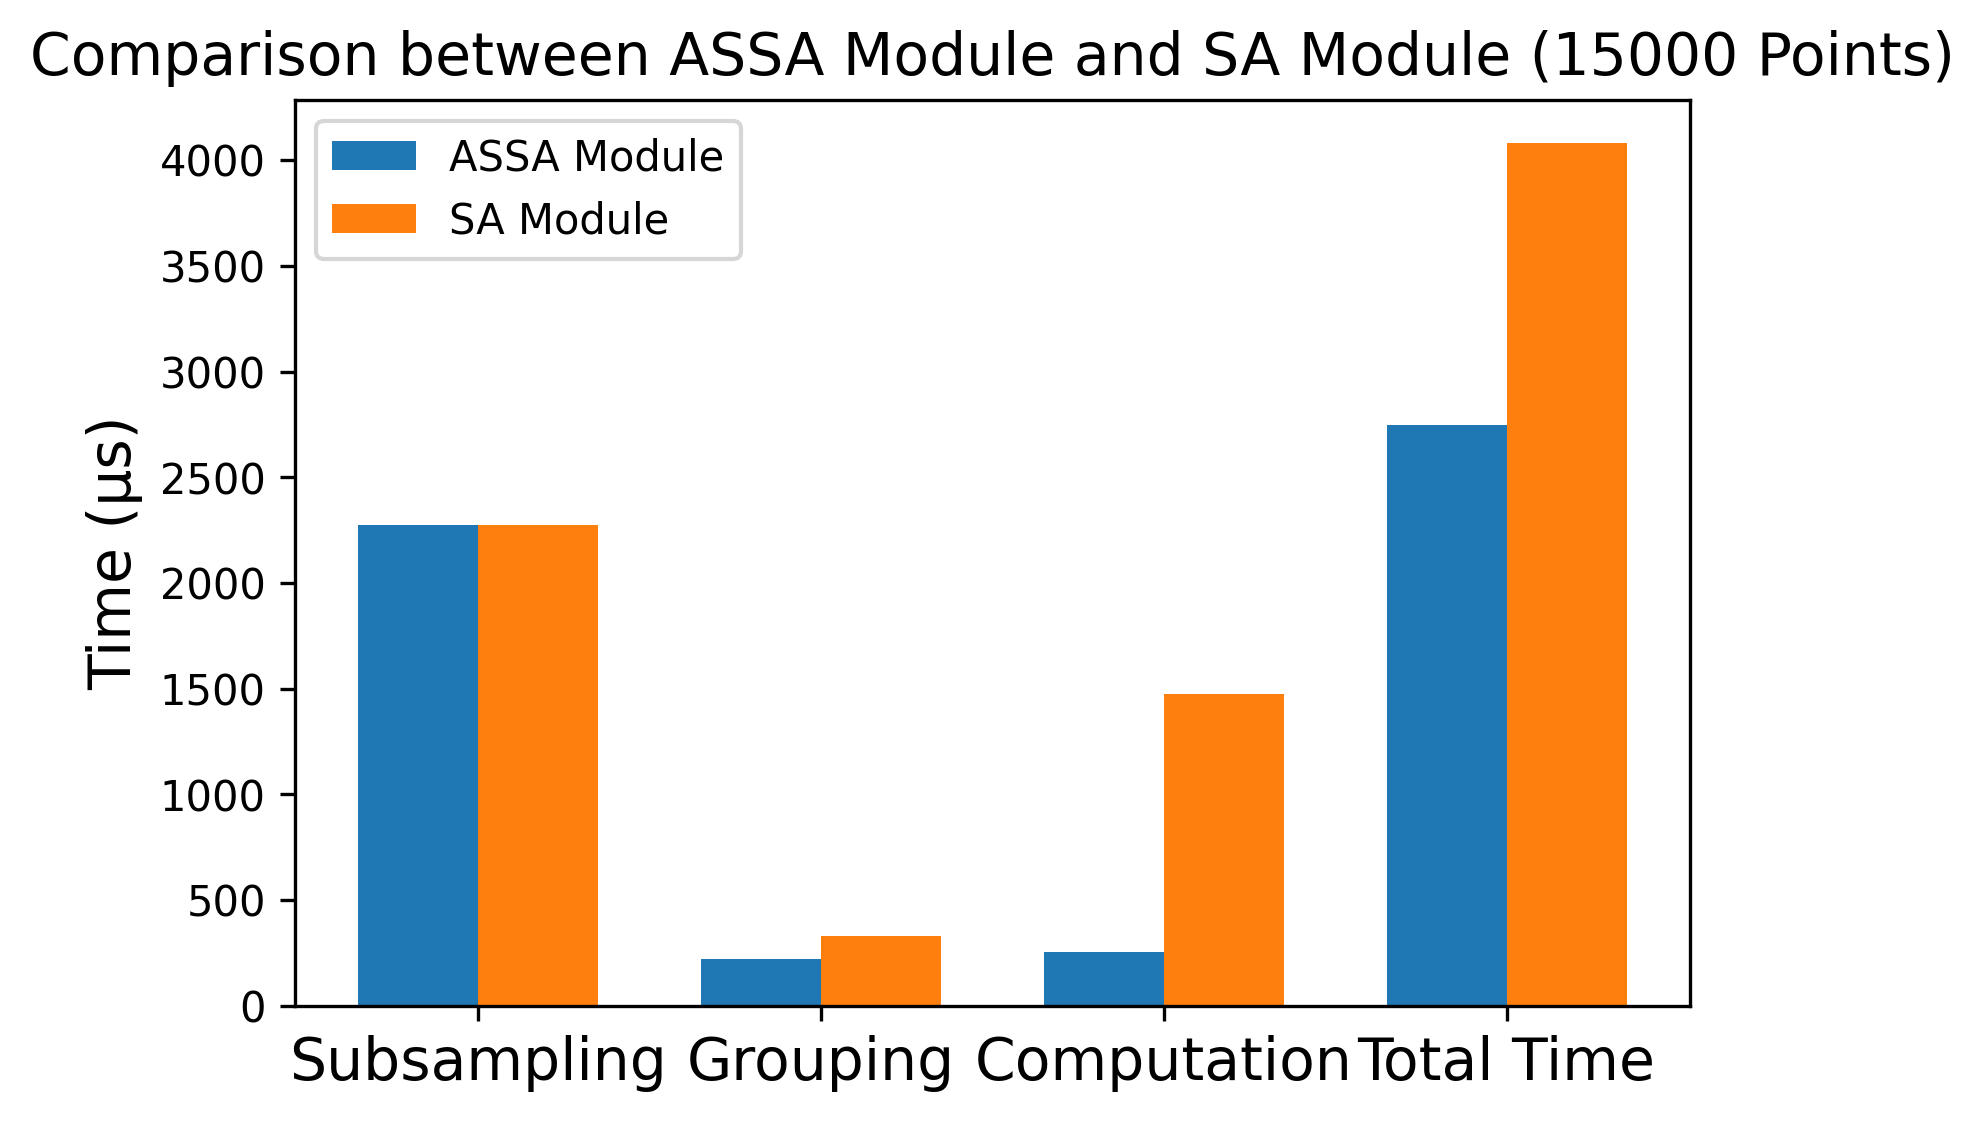}
        \caption{Latency decomposition (15,000 points)}
        \label{fig:latency_15k}
    \end{subfigure}%
\caption{
\textbf{Latency decomposition of proposed ASSA module compared with vanilla SA module}. 
}
\end{figure}

\section{Feature Patterns}
Following PointNet++ \cite{Qi2017PointNetDH}, we also visualize what has been learned by the first ASSA module. We create a voxel grid in space and aggregate local point sets that activate certain neurons the most in grid cells (highest 100 examples are used). Grid cells with high votes are kept and converted back to 3D point clouds, which represents the pattern that neuron recognizes. We use objects from ModelNet40 as examples. \figLabel \ref{fig:feature_pattern1} - \ref{fig:feature_pattern5} show the feature patterns before and after the first ASSA module of airplane, car, chair, table, lamp, and person. These figures show that the proposed ASSA module helps capture better geometric relationships.

\begin{figure}[!ht]

    \begin{subfigure}{6in}
    \centering
        \includegraphics[height=28mm]{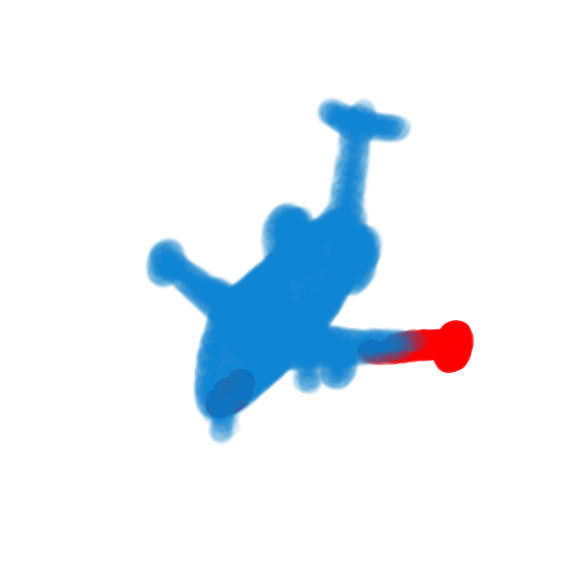}
        \includegraphics[height=28mm]{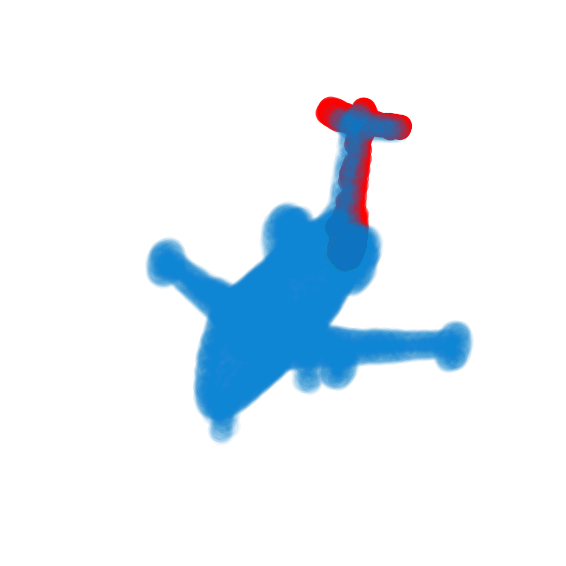}
        \includegraphics[height=28mm]{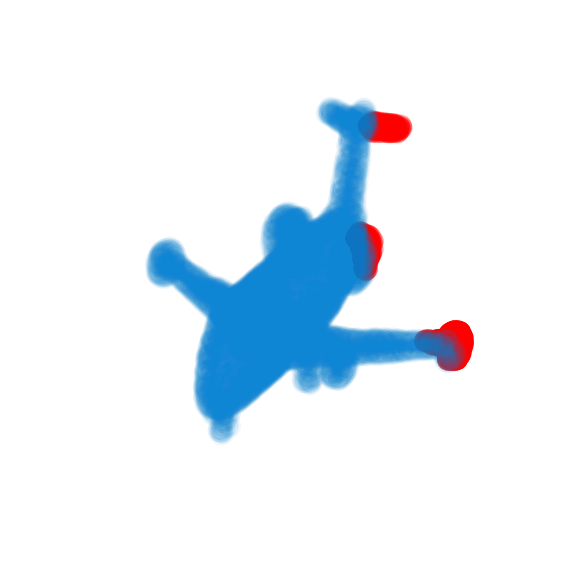}
        \includegraphics[height=28mm]{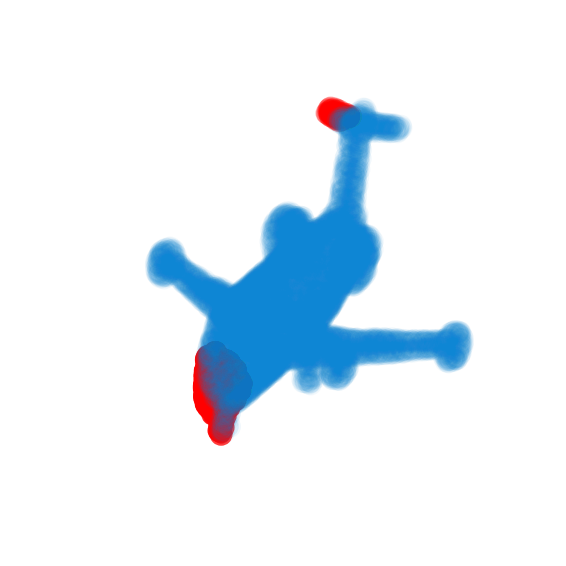}
        \includegraphics[height=28mm]{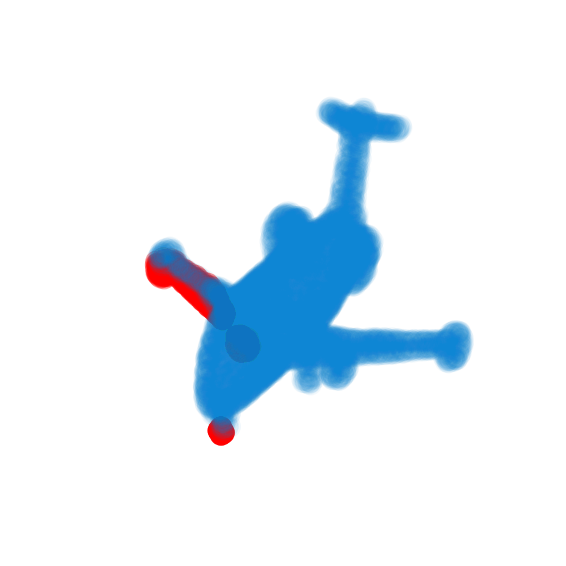}
        \caption{Feature Patterns Before ASSA Module}
    \end{subfigure}%

    \begin{subfigure}{6in}
    \centering
        \includegraphics[height=28mm]{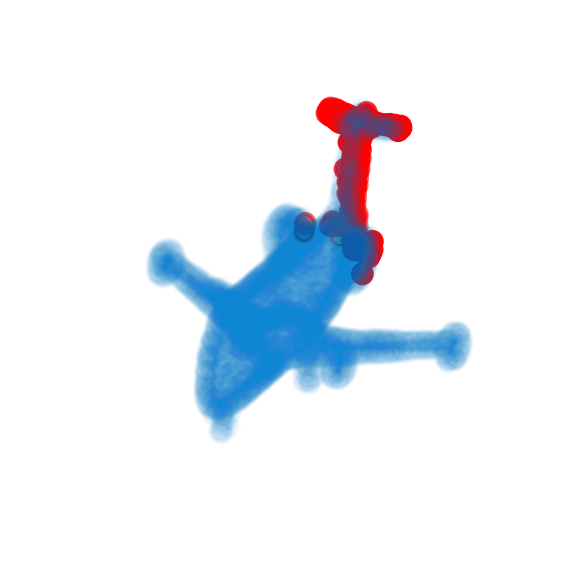}
        \includegraphics[height=28mm]{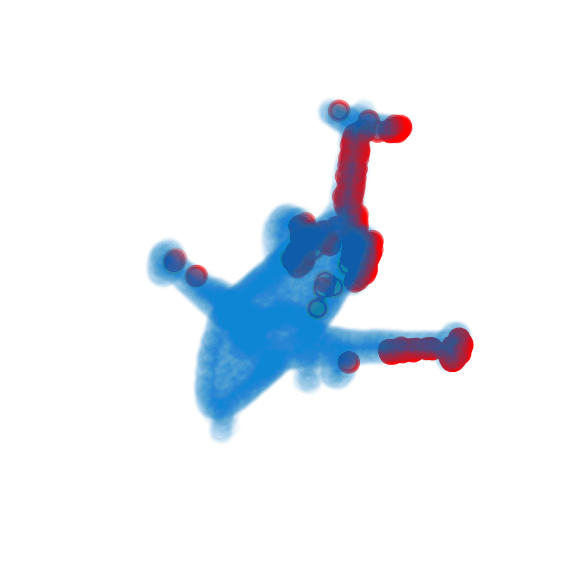}
        \includegraphics[height=28mm]{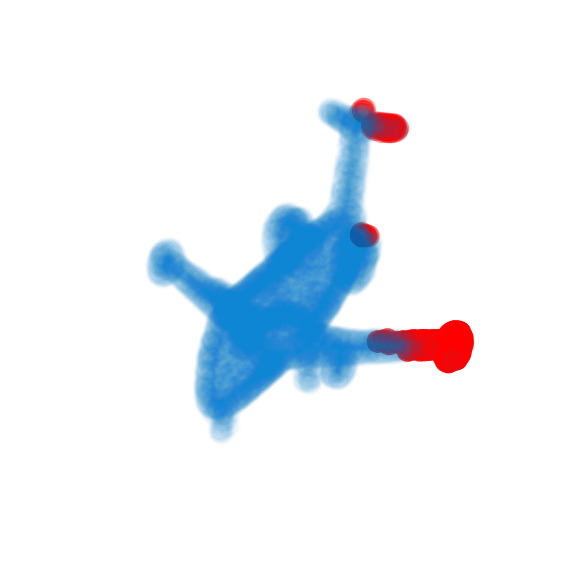}
        \includegraphics[height=28mm]{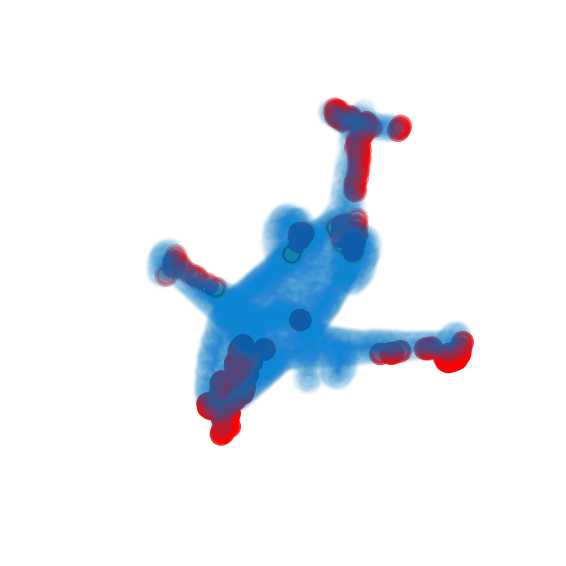}
        \includegraphics[height=28mm]{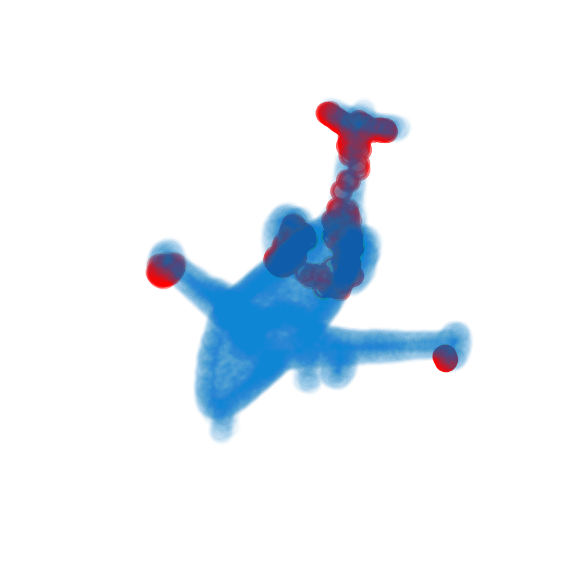}
    \end{subfigure}%
    
    \begin{subfigure}{6in}
    \centering
        \includegraphics[height=28mm]{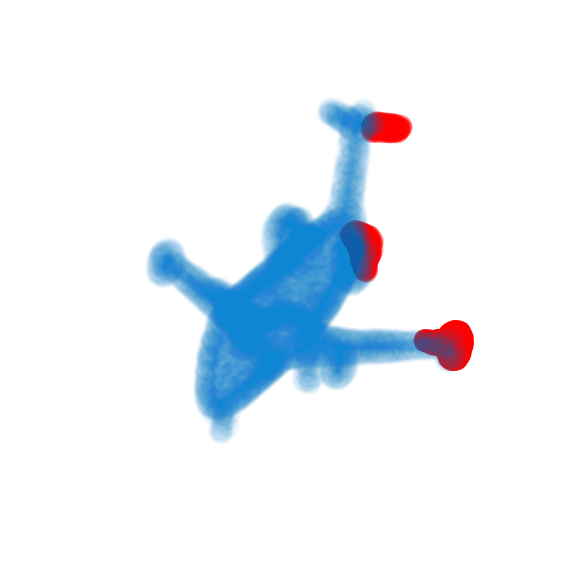}
        \includegraphics[height=28mm]{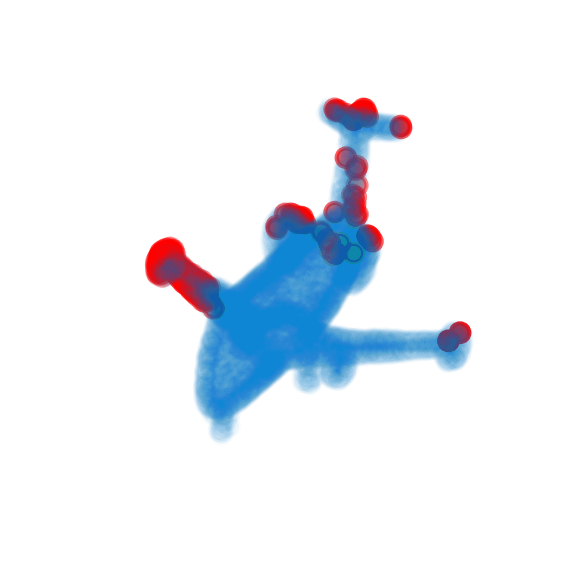}
        \includegraphics[height=28mm]{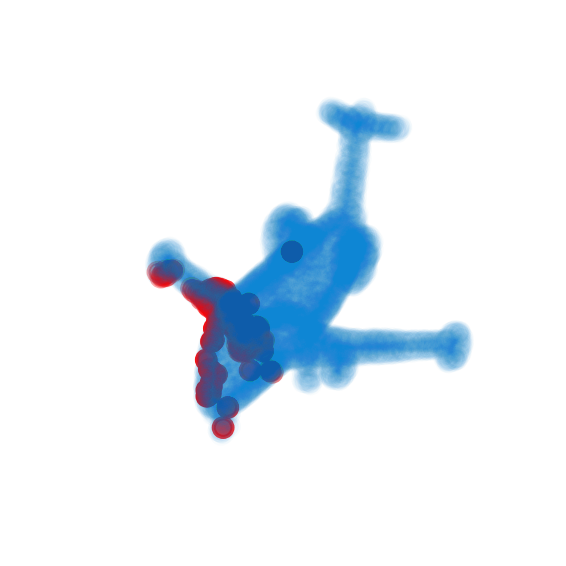}
        \includegraphics[height=28mm]{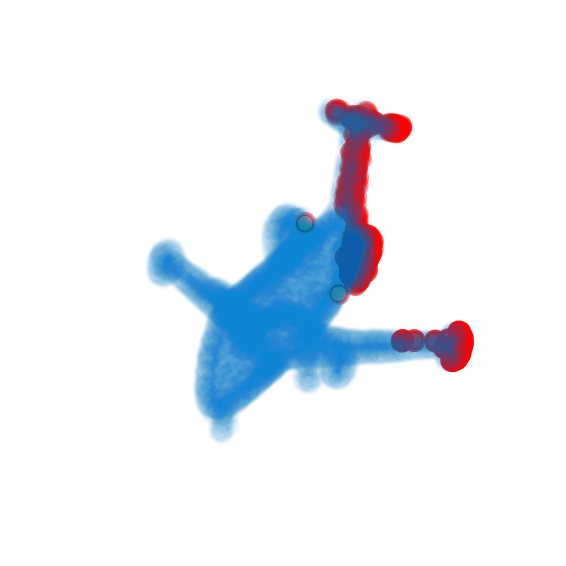}
        \includegraphics[height=28mm]{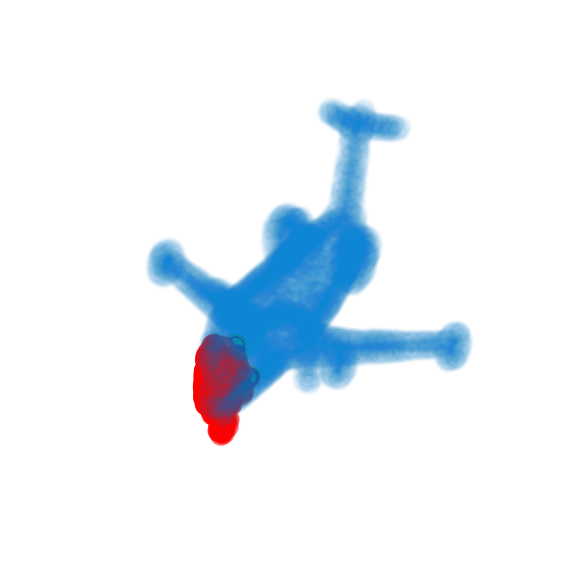}
    \end{subfigure}%
    
    \begin{subfigure}{6in}
    \centering
        \includegraphics[height=28mm]{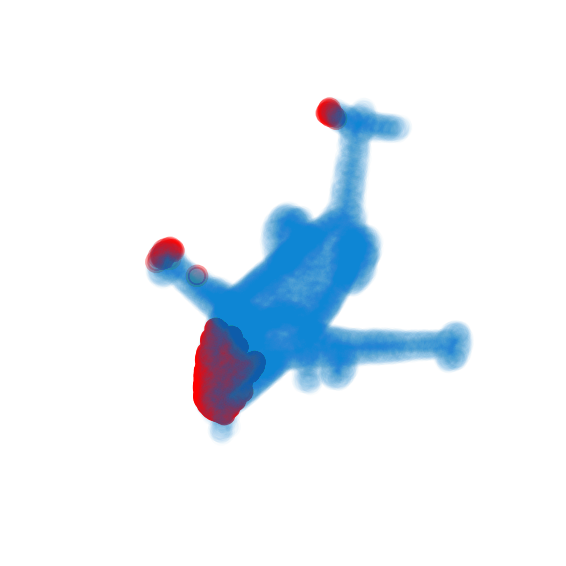}
        \includegraphics[height=28mm]{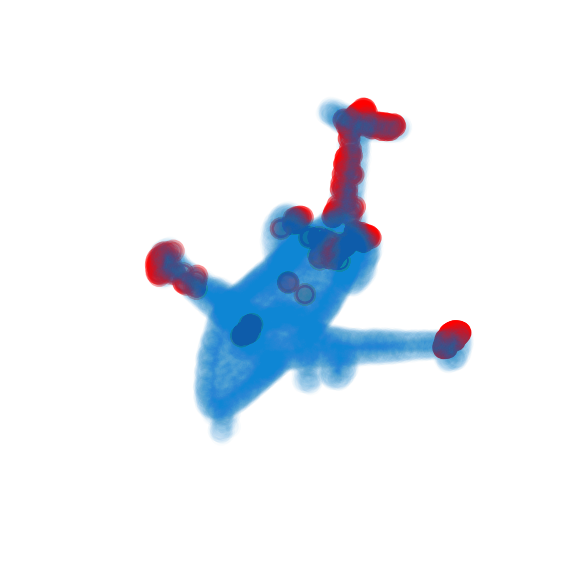}
        \includegraphics[height=28mm]{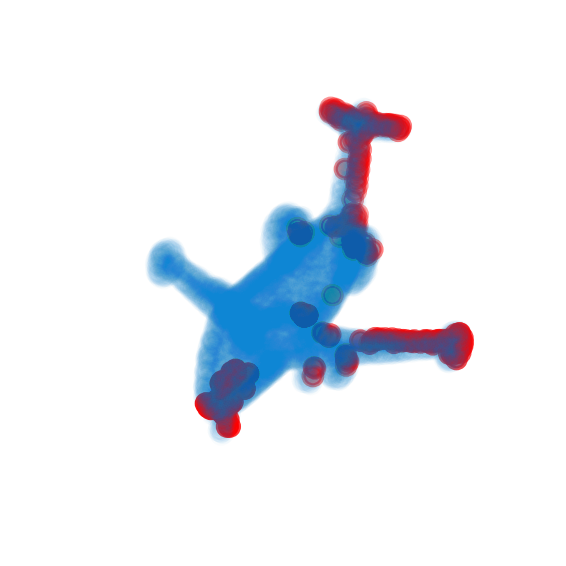}
        \includegraphics[height=28mm]{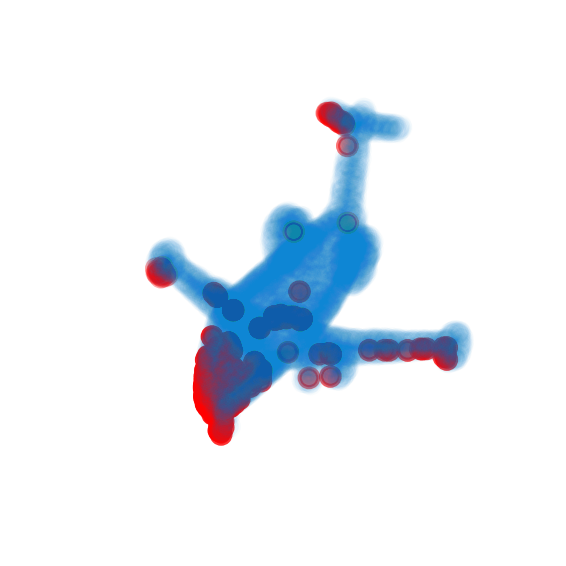}
        \includegraphics[height=28mm]{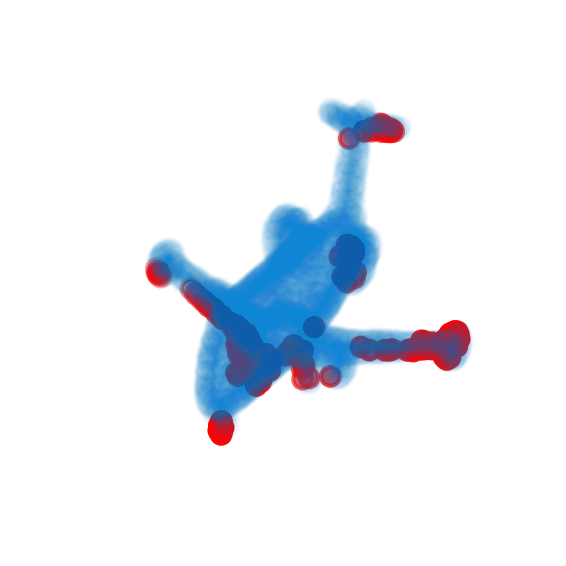}
        \caption{Feature Patterns After ASSA Module}
        
    \end{subfigure}%

\caption{Airplane feature patterns visualization}
\label{fig:feature_pattern1}
\end{figure}

\begin{figure}[!ht]

    \begin{subfigure}{6in}
    \centering
        \includegraphics[height=28mm]{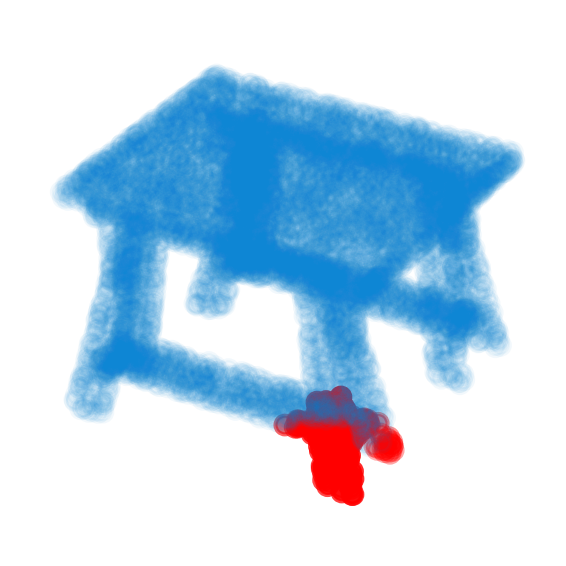}
        \includegraphics[height=28mm]{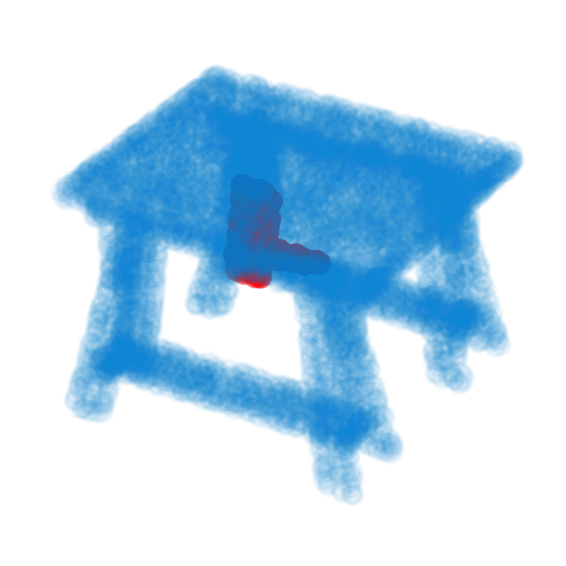}
        \includegraphics[height=28mm]{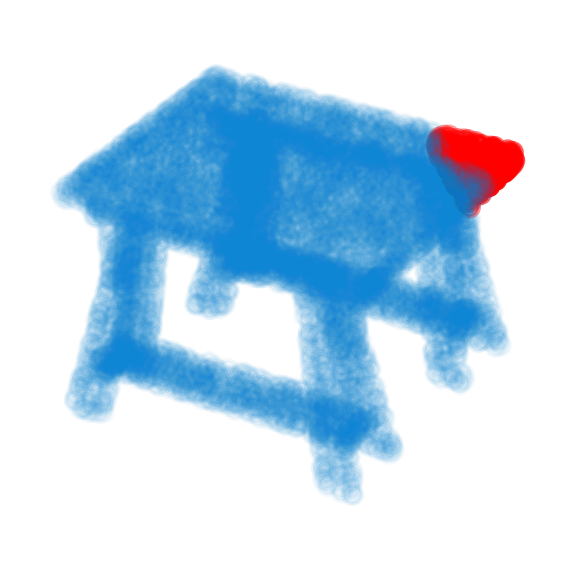}
        \includegraphics[height=28mm]{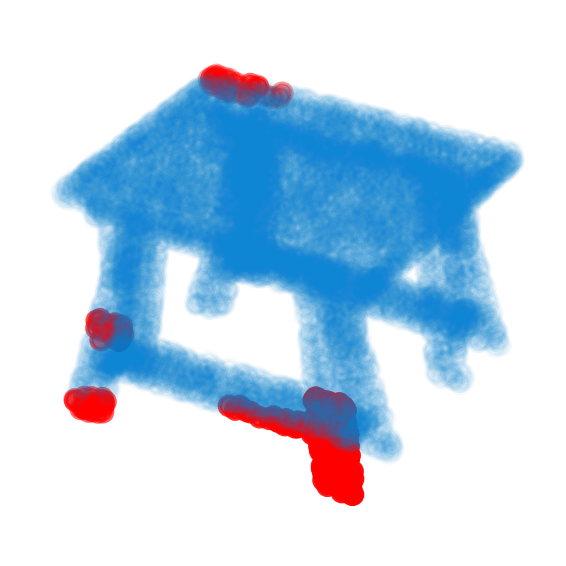}
        \includegraphics[height=28mm]{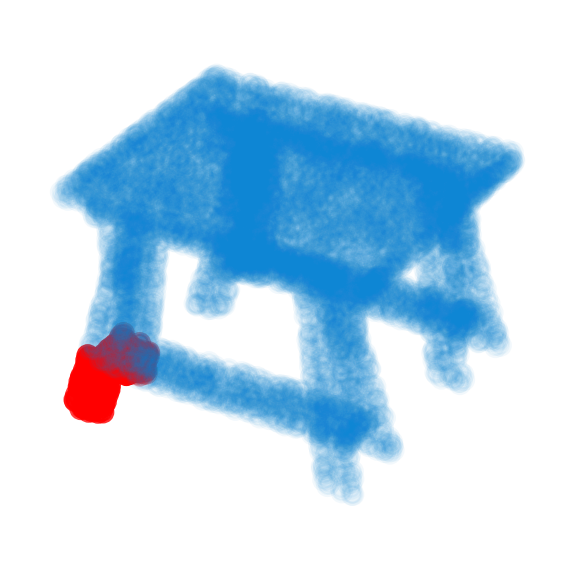}
        \caption{Feature Patterns Before ASSA Module}
    \end{subfigure}%

    \begin{subfigure}{6in}
    \centering
        \includegraphics[height=28mm]{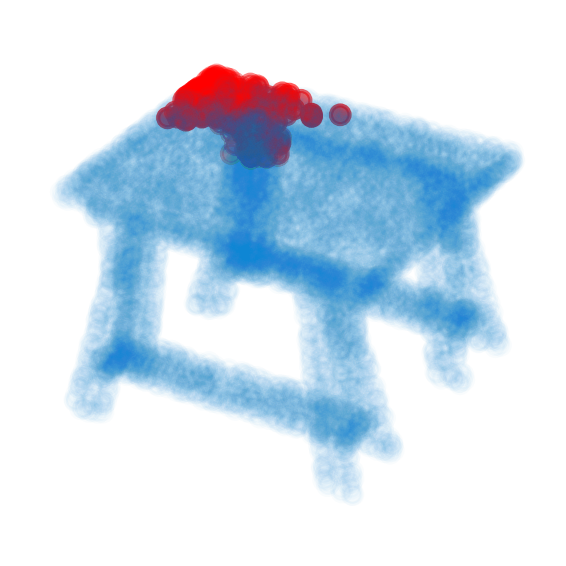}
        \includegraphics[height=28mm]{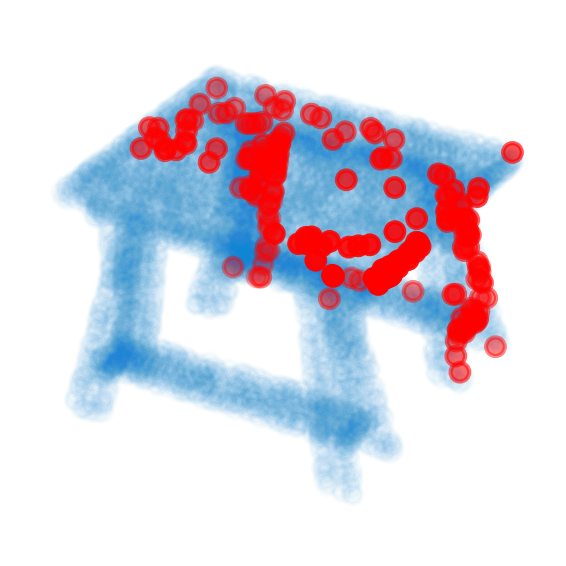}
        \includegraphics[height=28mm]{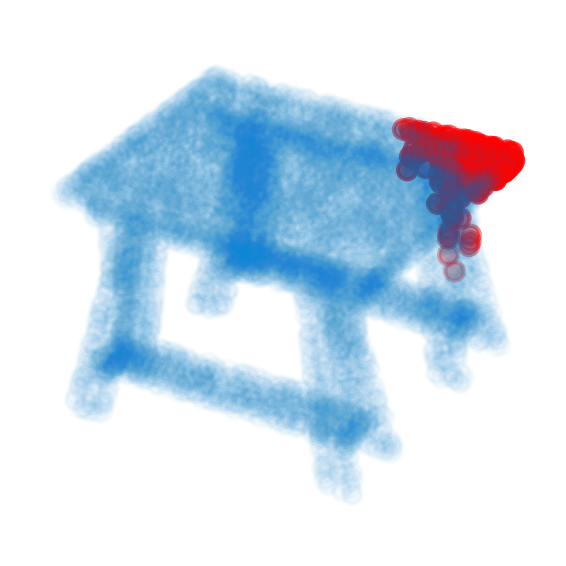}
        \includegraphics[height=28mm]{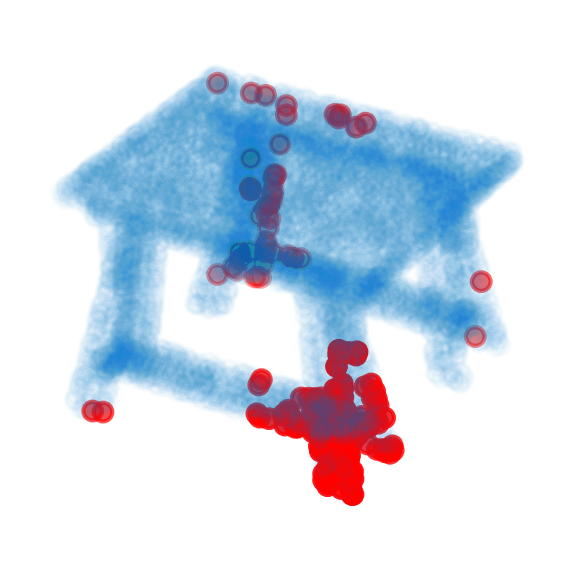}
        \includegraphics[height=28mm]{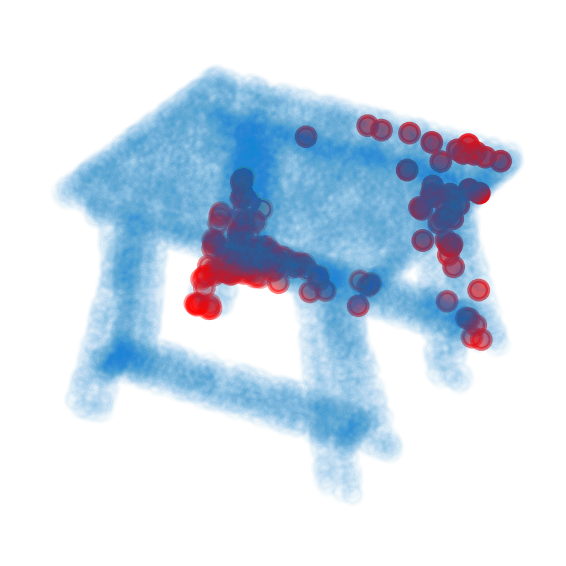}
    \end{subfigure}%
    
    \begin{subfigure}{6in}
    \centering
        \includegraphics[height=28mm]{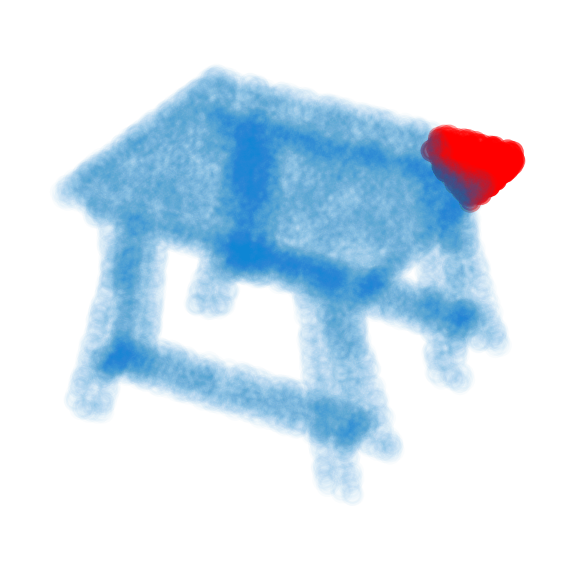}
        \includegraphics[height=28mm]{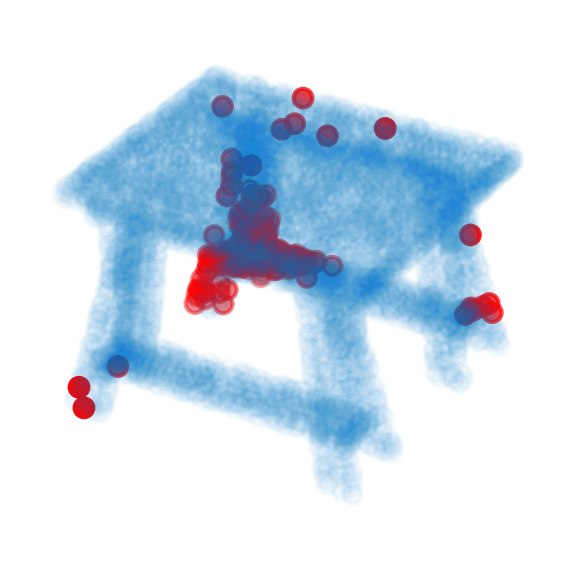}
        \includegraphics[height=28mm]{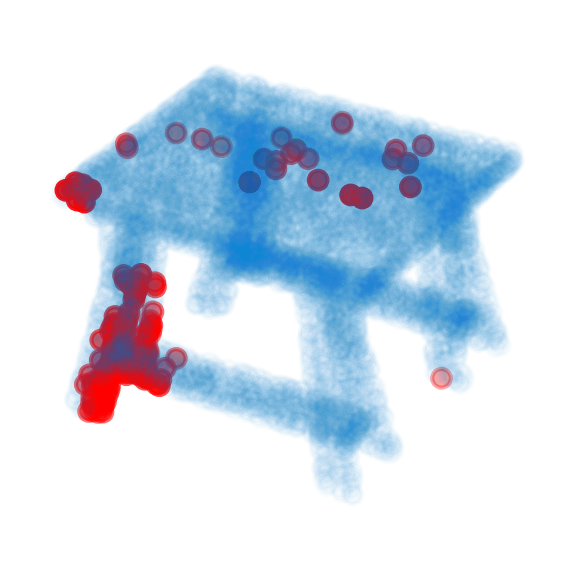}
        \includegraphics[height=28mm]{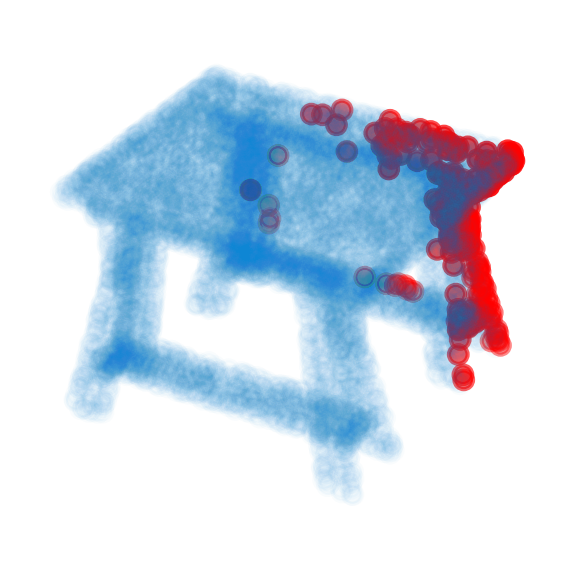}
        \includegraphics[height=28mm]{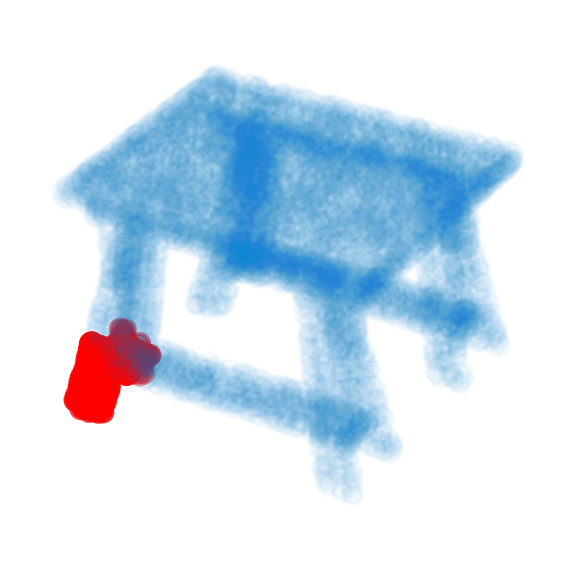}
    \end{subfigure}%
    
    \begin{subfigure}{6in}
    \centering
        \includegraphics[height=28mm]{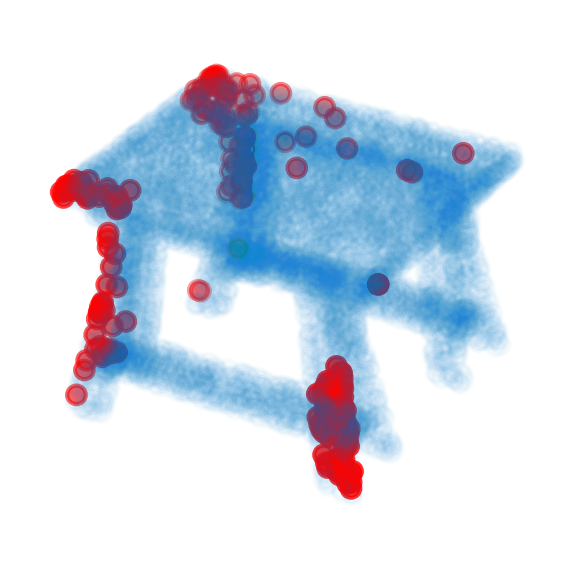}
        \includegraphics[height=28mm]{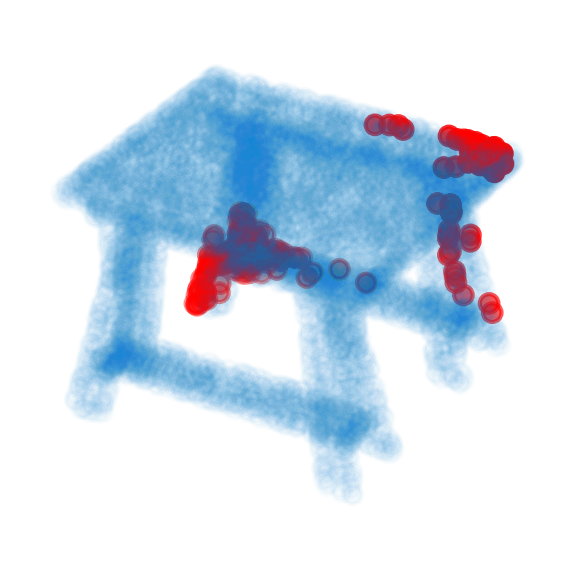}
        \includegraphics[height=28mm]{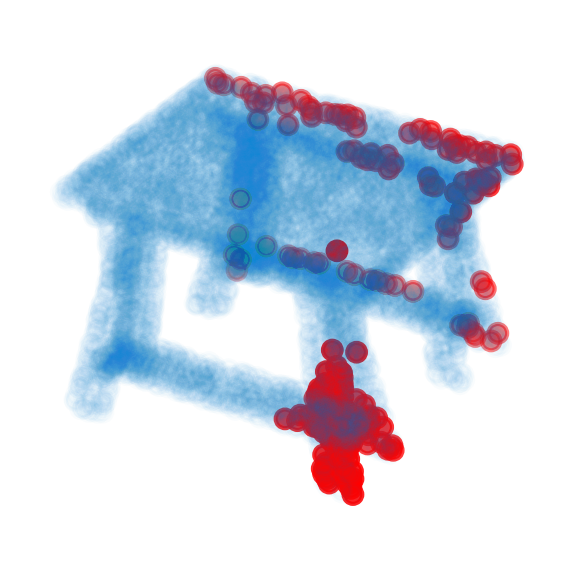}
        \includegraphics[height=28mm]{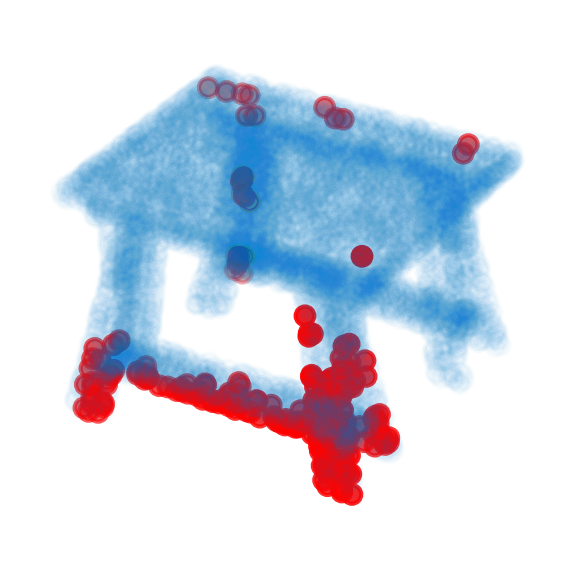}
        \includegraphics[height=28mm]{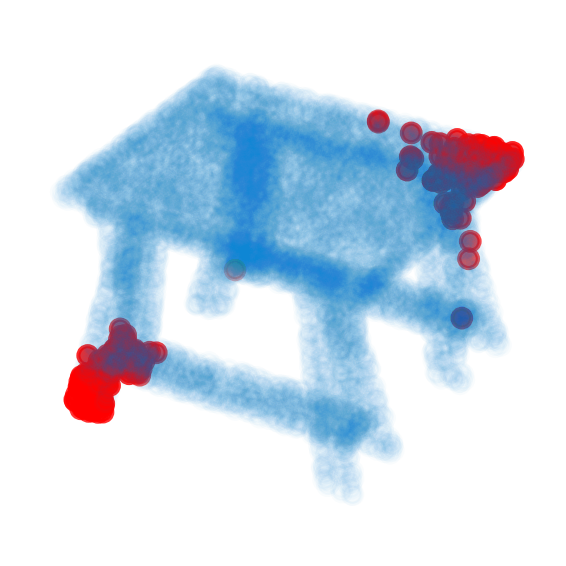}
        \caption{Feature Patterns After ASSA Module}
        
    \end{subfigure}%

\caption{Table feature patterns visualization}
\label{fig:feature_pattern2}
\end{figure}

\begin{figure}[!ht]

    \begin{subfigure}{6in}
    \centering
        \includegraphics[height=28mm]{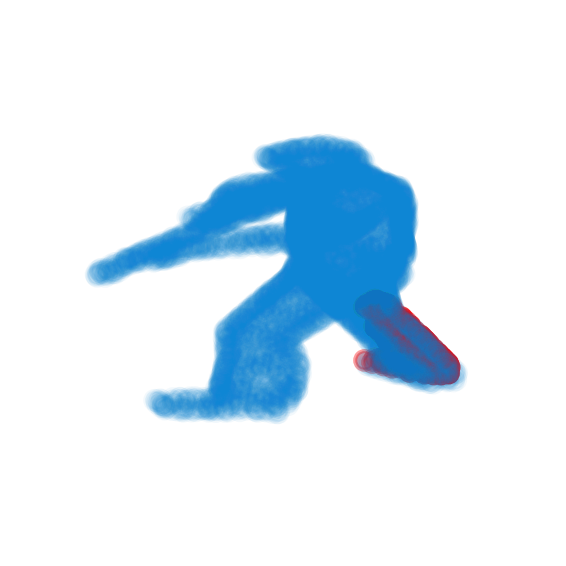}
        \includegraphics[height=28mm]{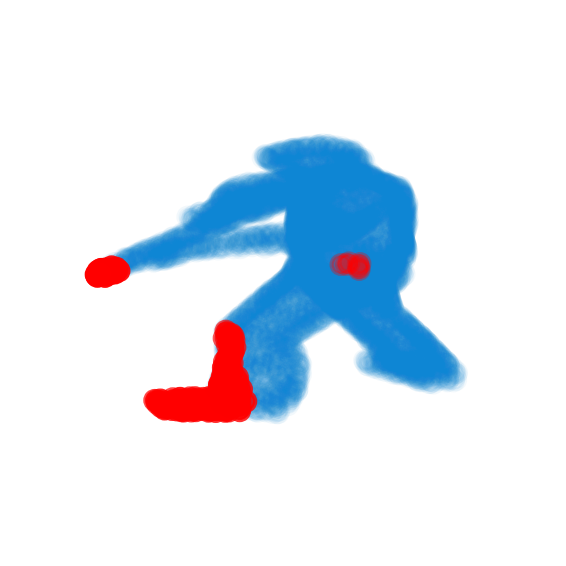}
        \includegraphics[height=28mm]{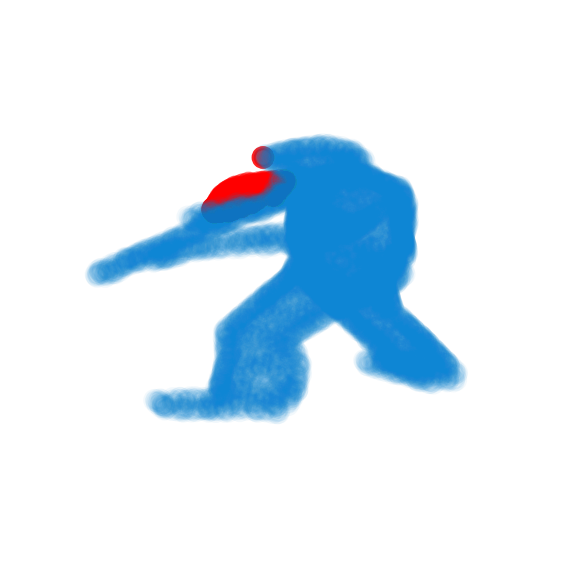}
        \includegraphics[height=28mm]{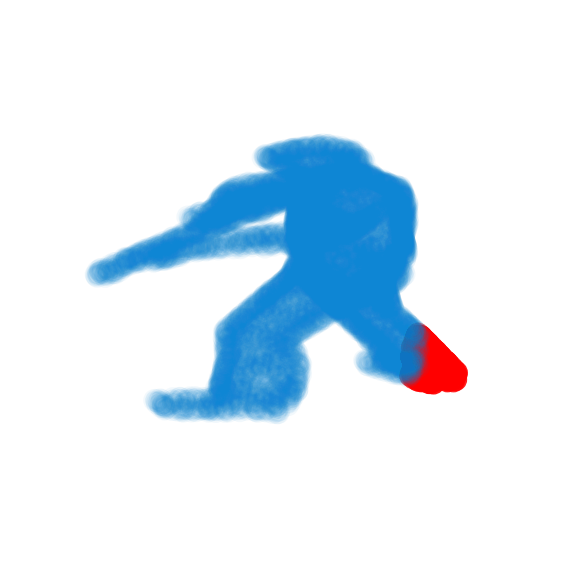}
        \includegraphics[height=28mm]{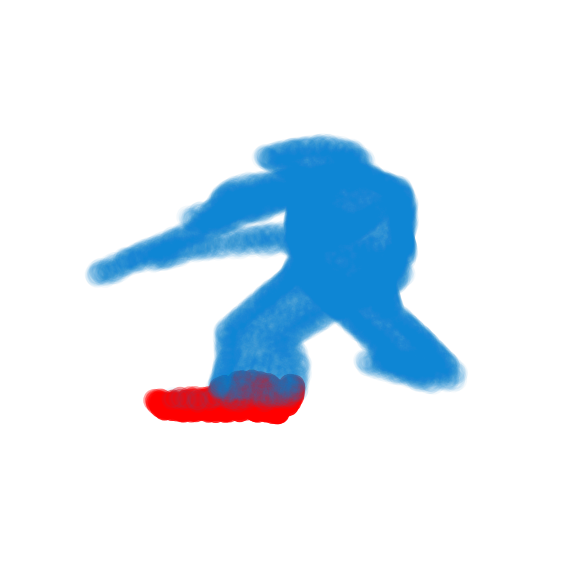}
        \caption{Feature Patterns Before ASSA Module}
    \end{subfigure}%

    \begin{subfigure}{6in}
    \centering
        \includegraphics[height=28mm]{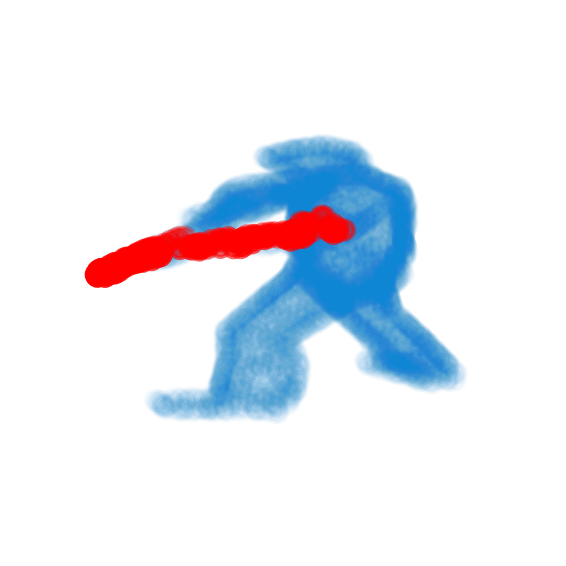}
        \includegraphics[height=28mm]{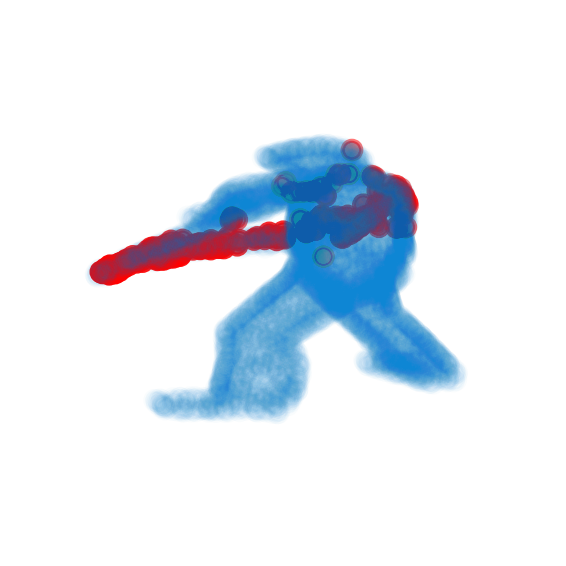}
        \includegraphics[height=28mm]{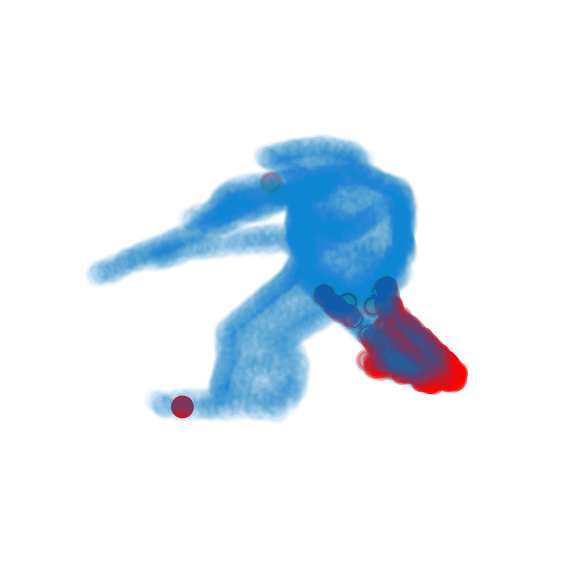}
        \includegraphics[height=28mm]{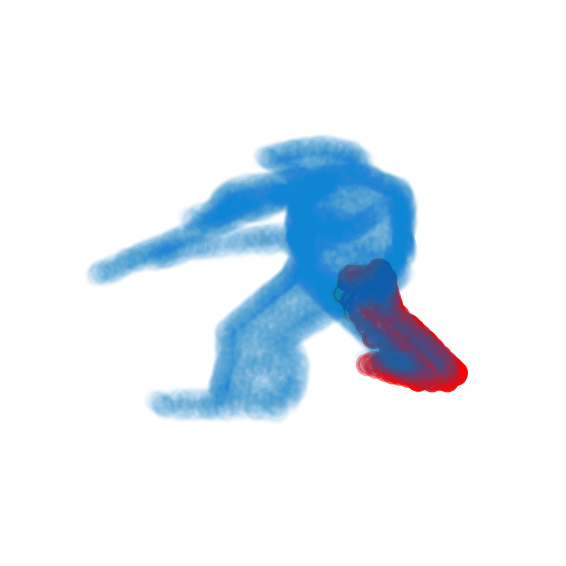}
        \includegraphics[height=28mm]{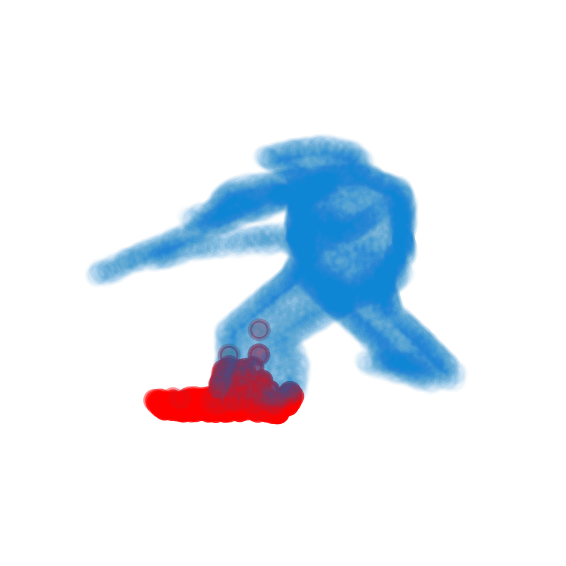}
    \end{subfigure}%
    
    \begin{subfigure}{6in}
    \centering
        \includegraphics[height=28mm]{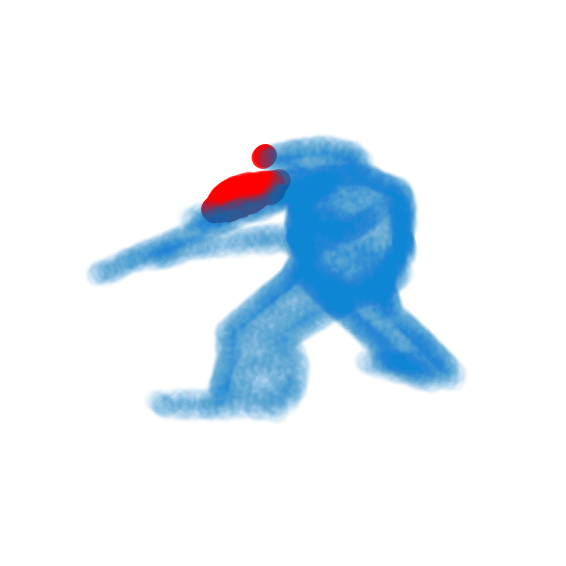}
        \includegraphics[height=28mm]{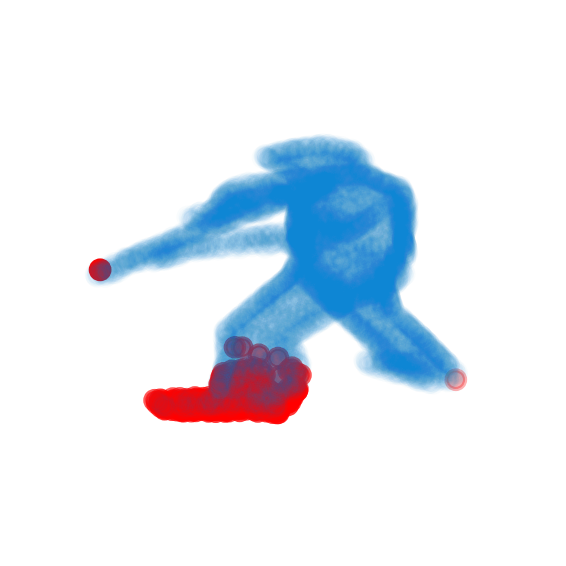}
        \includegraphics[height=28mm]{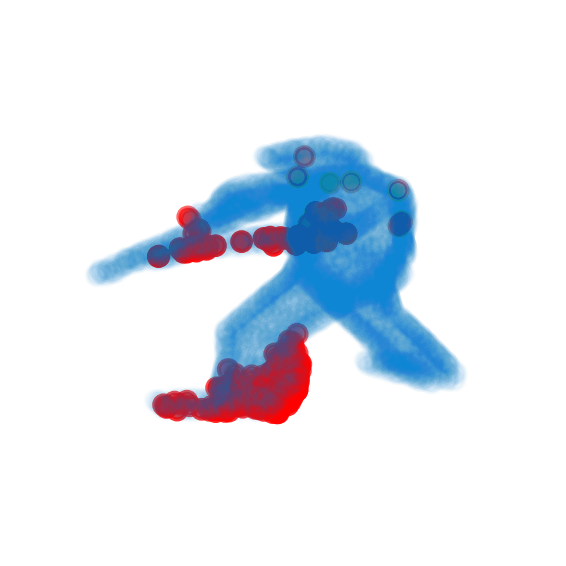}
        \includegraphics[height=28mm]{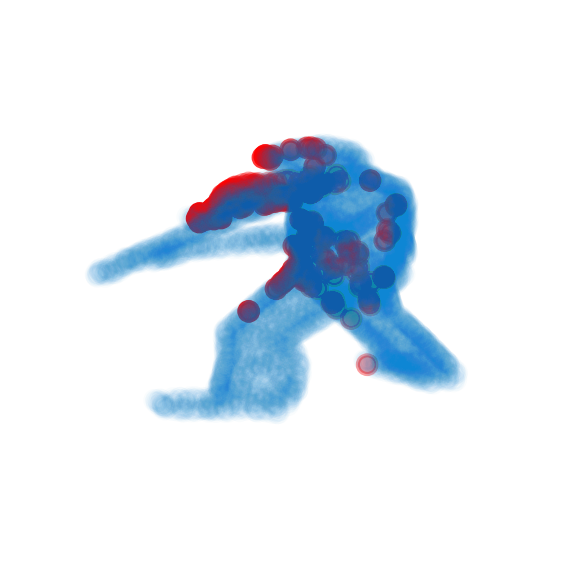}
        \includegraphics[height=28mm]{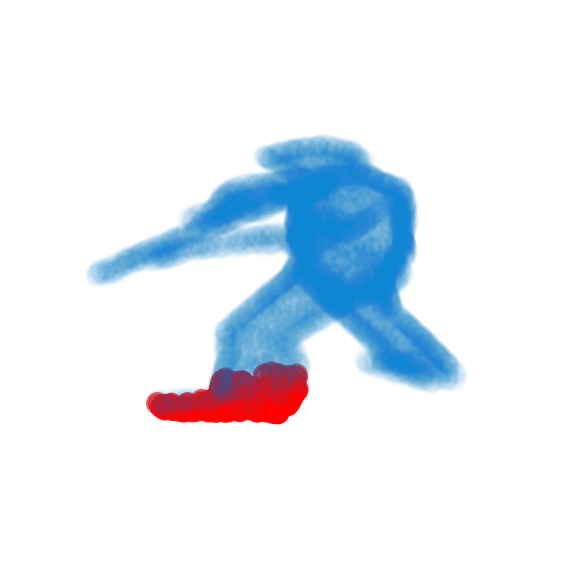}
    \end{subfigure}%
    
    \begin{subfigure}{6in}
    \centering
        \includegraphics[height=28mm]{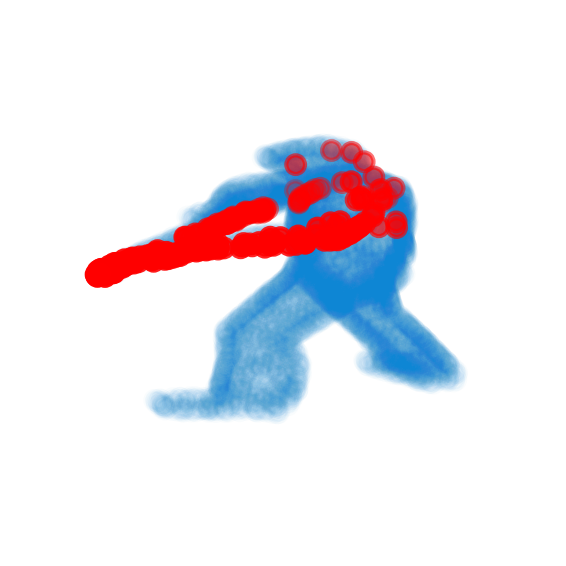}
        \includegraphics[height=28mm]{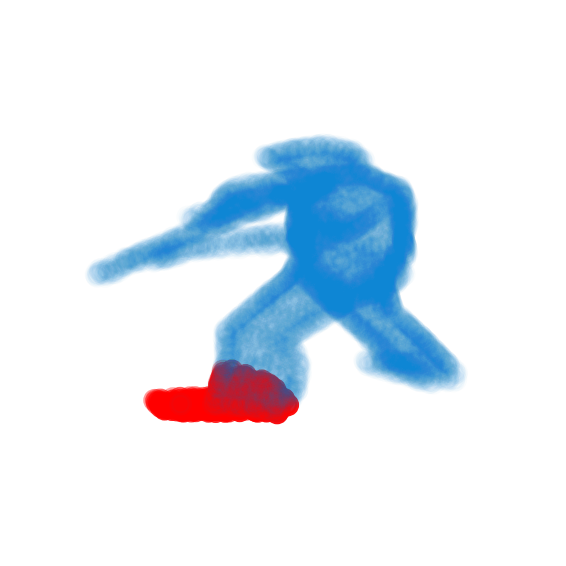}
        \includegraphics[height=28mm]{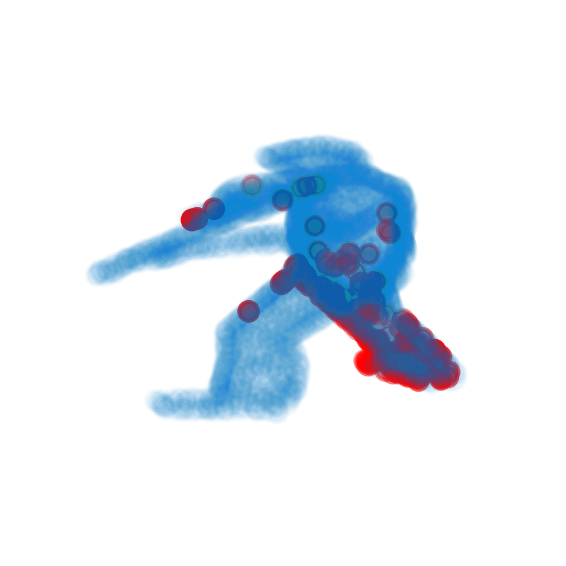}
        \includegraphics[height=28mm]{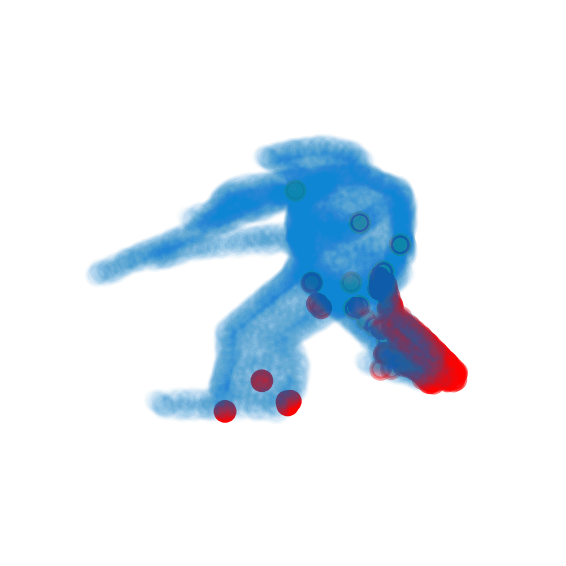}
        \includegraphics[height=28mm]{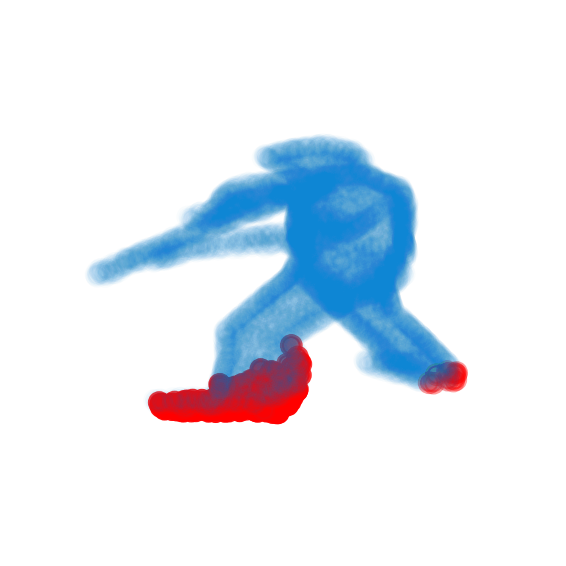}
        \caption{Feature Patterns After ASSA Module}
        
    \end{subfigure}%

\caption{Human feature patterns visualization}
\label{fig:feature_pattern3}
\end{figure}

\begin{figure}[!ht]

    \begin{subfigure}{6in}
    \centering
        \includegraphics[height=28mm]{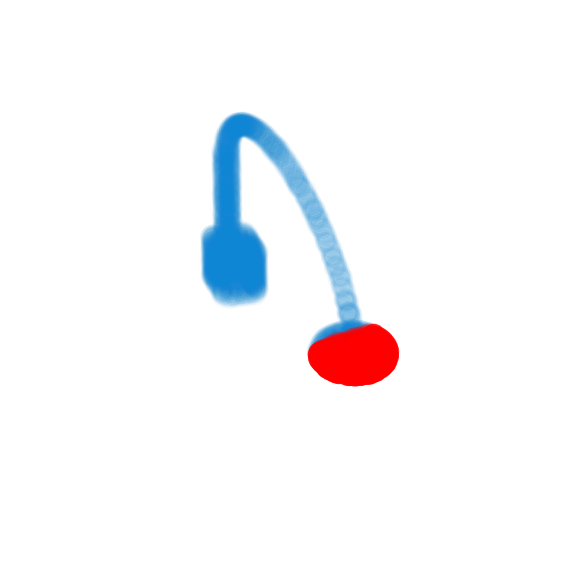}
        \includegraphics[height=28mm]{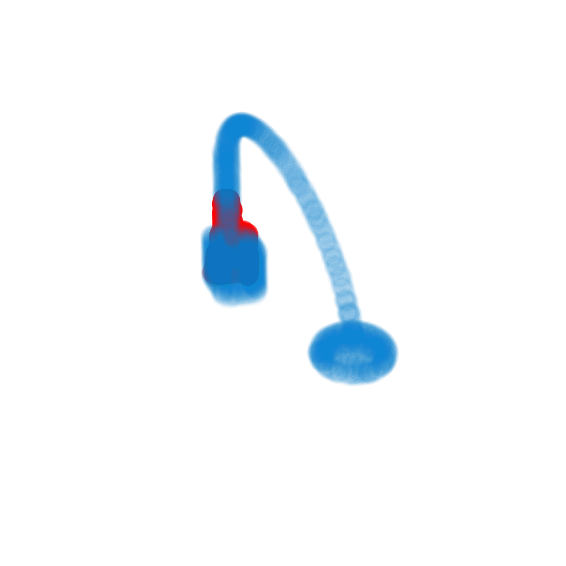}
        \includegraphics[height=28mm]{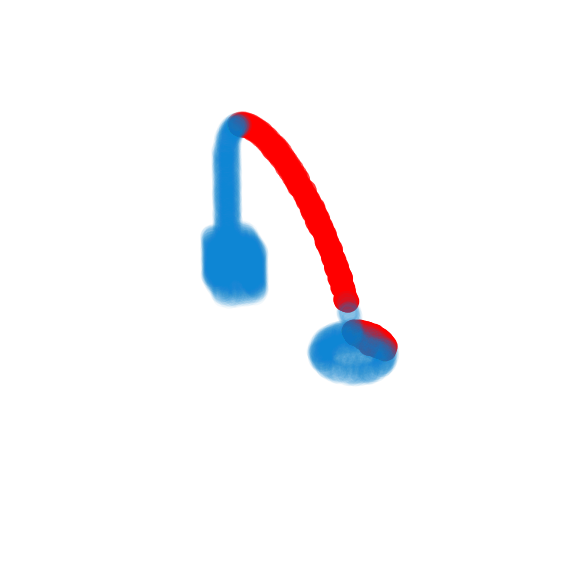}
        \includegraphics[height=28mm]{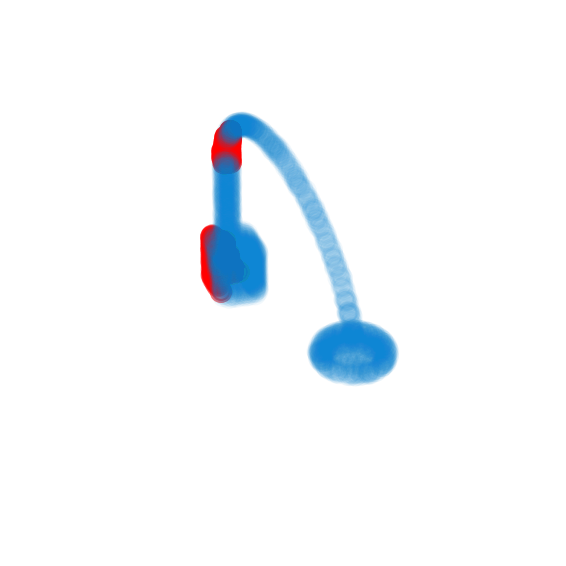}
        \includegraphics[height=28mm]{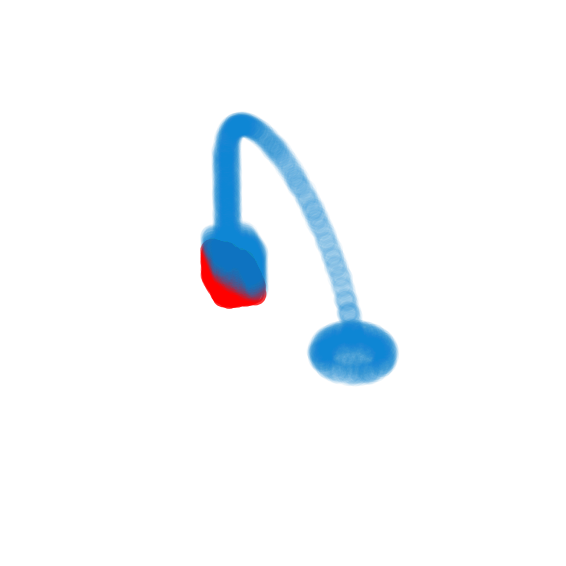}
        \caption{Feature Patterns Before ASSA Module}
    \end{subfigure}%

    \begin{subfigure}{6in}
    \centering
        \includegraphics[height=28mm]{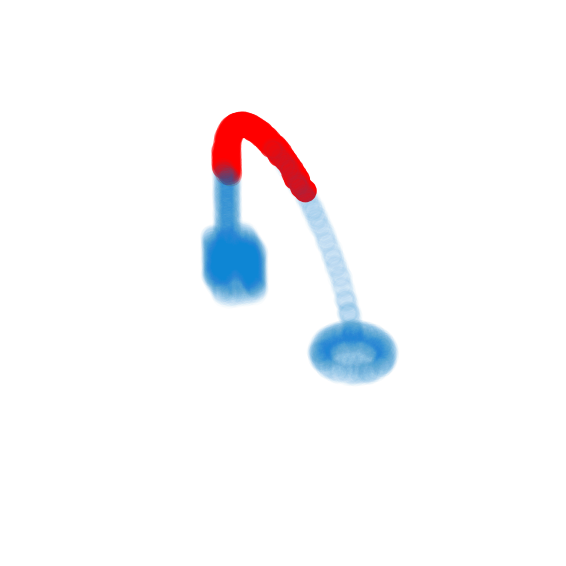}
        \includegraphics[height=28mm]{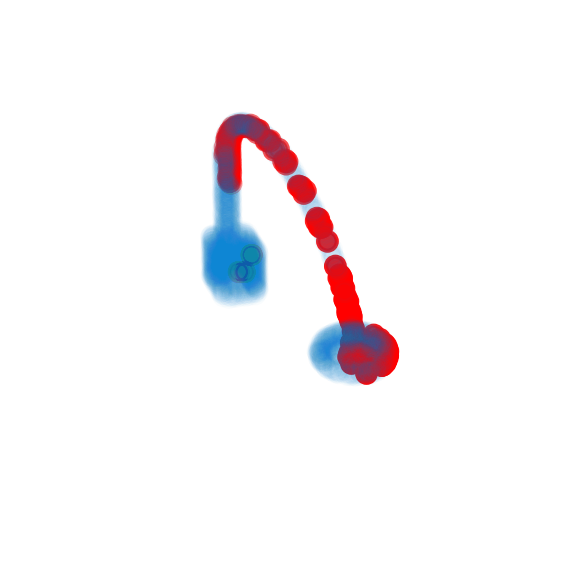}
        \includegraphics[height=28mm]{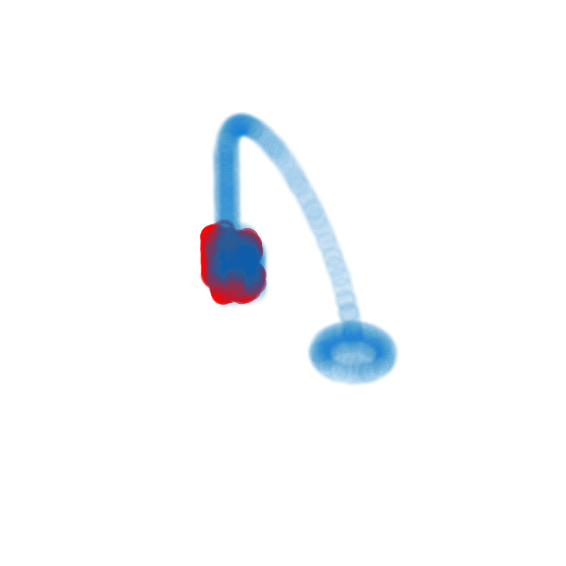}
        \includegraphics[height=28mm]{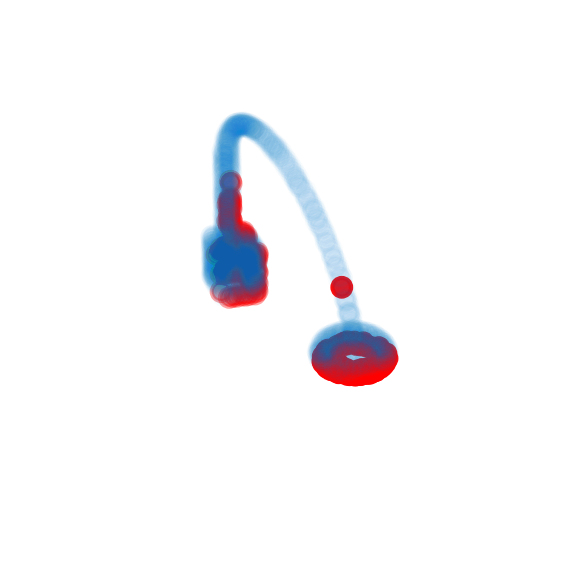}
        \includegraphics[height=28mm]{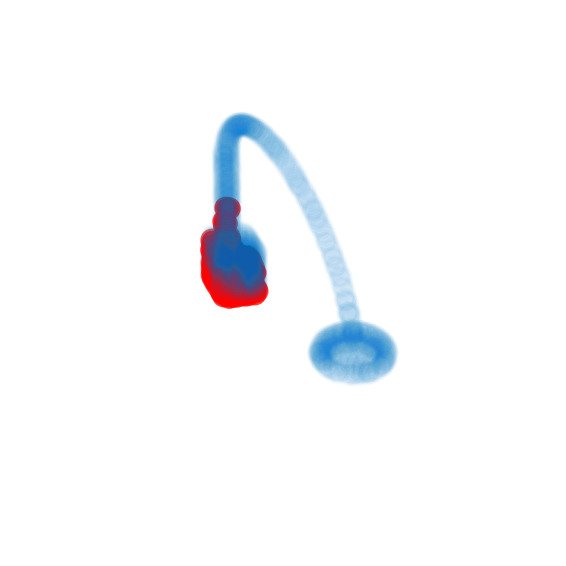}
    \end{subfigure}%
    
    \begin{subfigure}{6in}
    \centering
        \includegraphics[height=28mm]{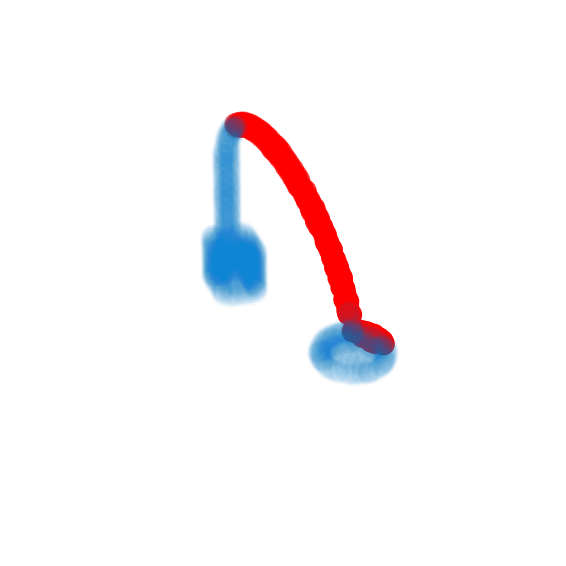}
        \includegraphics[height=28mm]{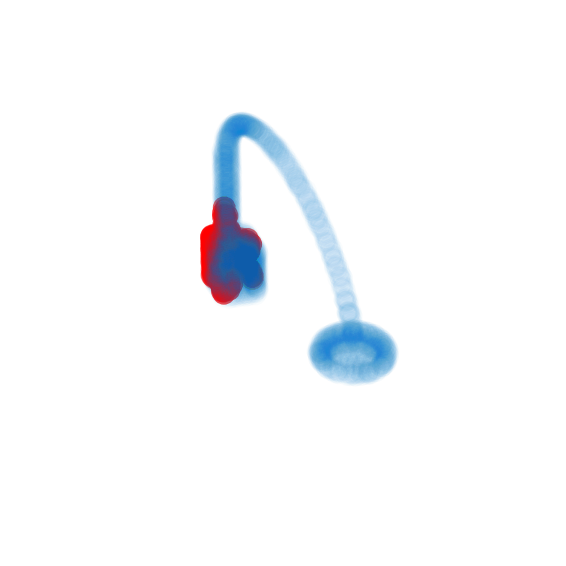}
        \includegraphics[height=28mm]{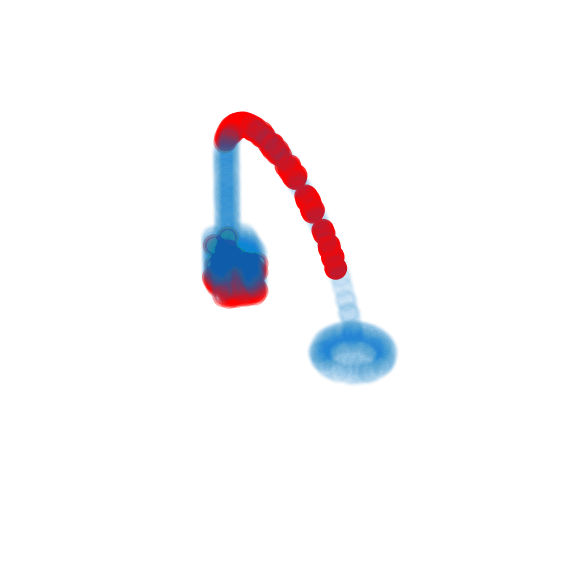}
        \includegraphics[height=28mm]{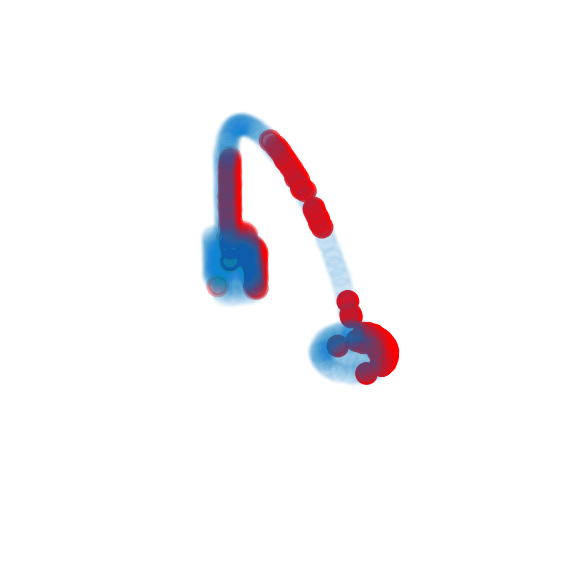}
        \includegraphics[height=28mm]{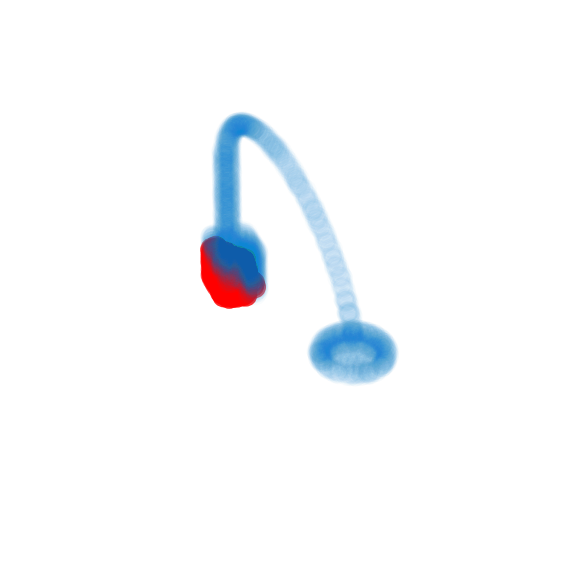}
    \end{subfigure}%
    
    \begin{subfigure}{6in}
    \centering
        \includegraphics[height=28mm]{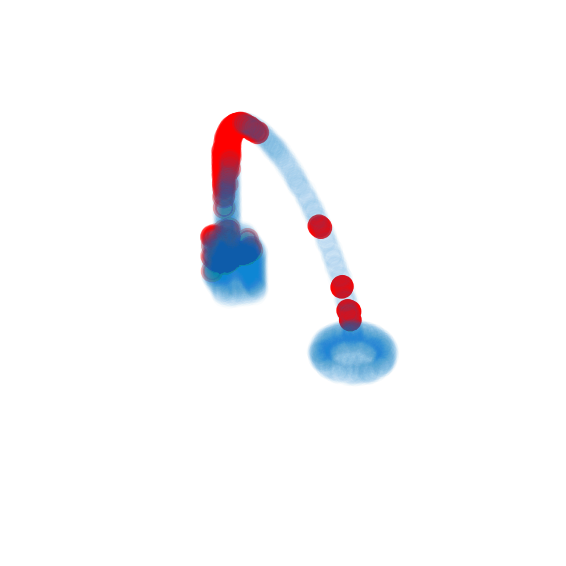}
        \includegraphics[height=28mm]{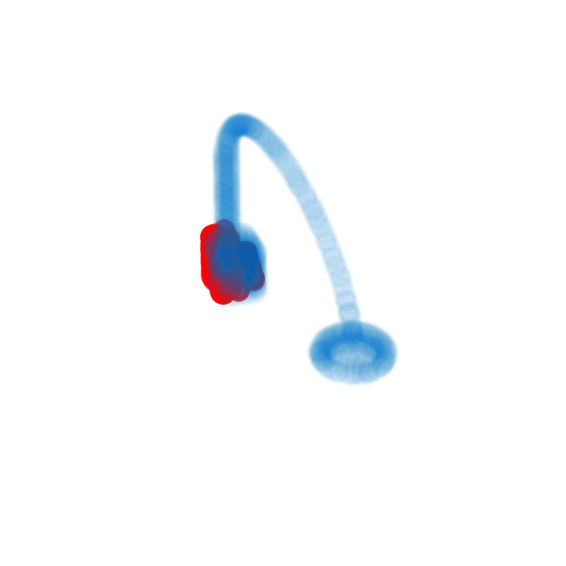}
        \includegraphics[height=28mm]{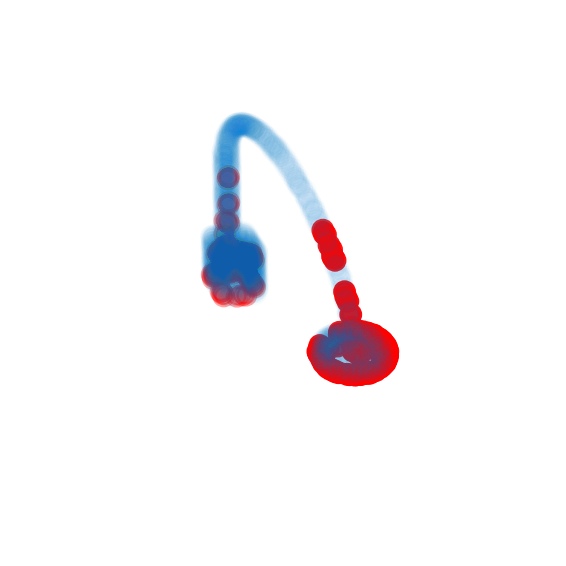}
        \includegraphics[height=28mm]{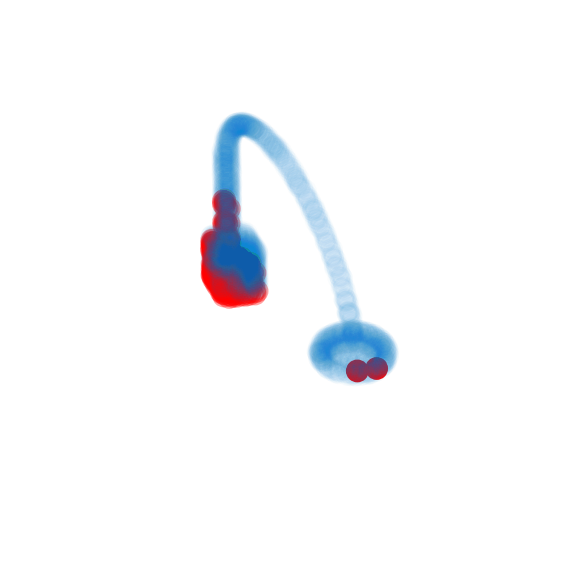}
        \includegraphics[height=28mm]{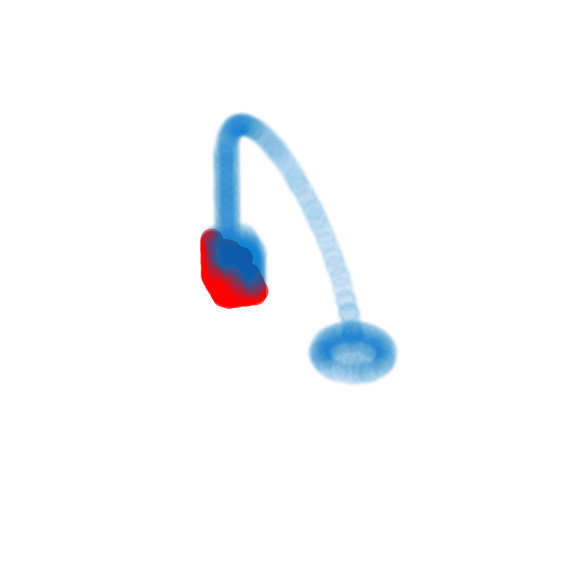}
        \caption{Feature Patterns After ASSA Module}
        
    \end{subfigure}%

\caption{Lamp feature patterns visualization}
\label{fig:feature_pattern4}
\end{figure}

\begin{figure}[!ht]

    \begin{subfigure}{6in}
    \centering
        \includegraphics[height=28mm]{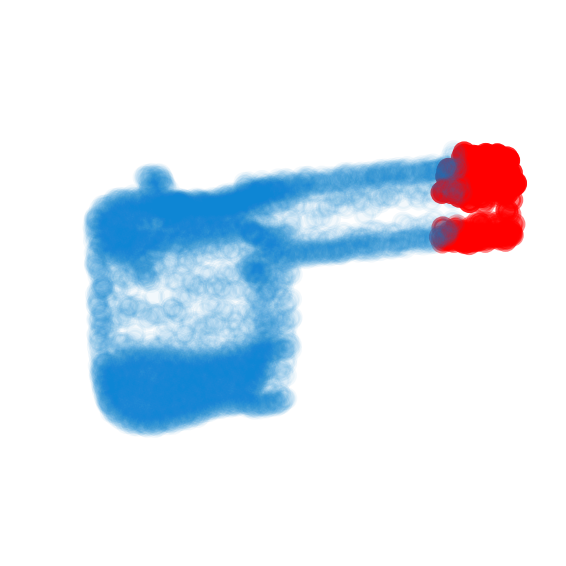}
        \includegraphics[height=28mm]{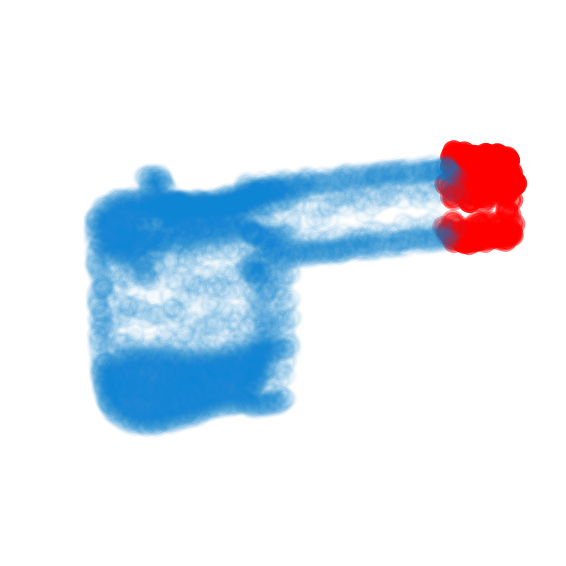}
        \includegraphics[height=28mm]{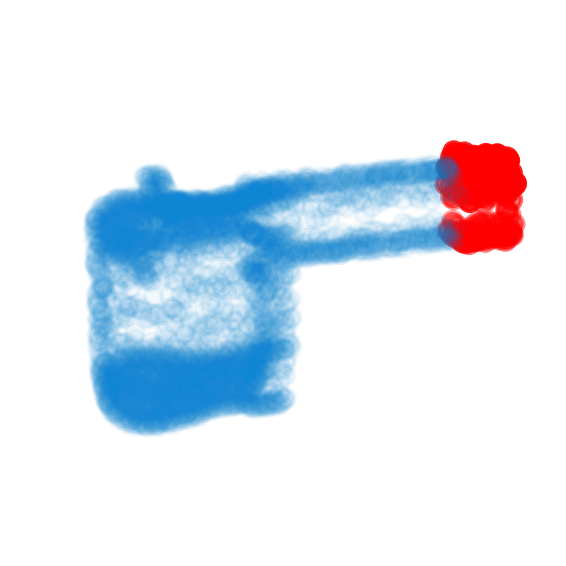}
        \includegraphics[height=28mm]{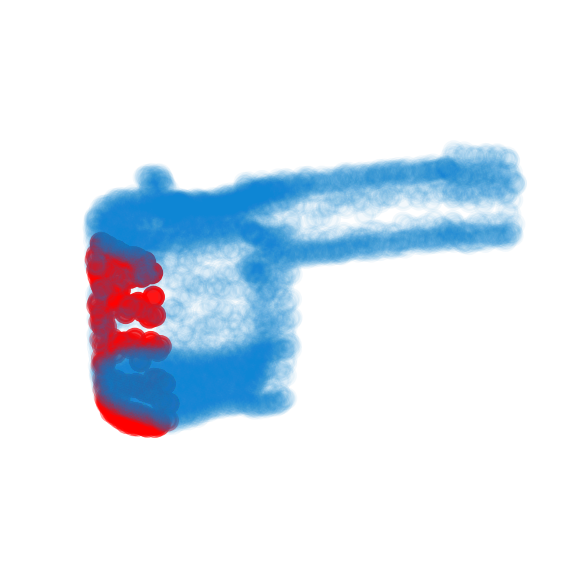}
        \includegraphics[height=28mm]{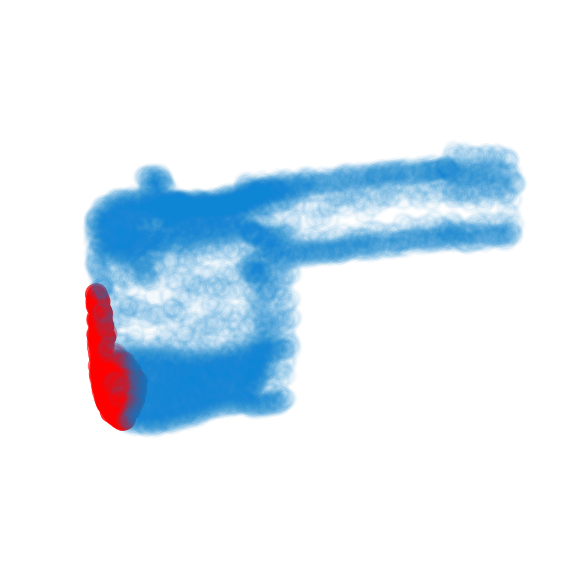}
        \caption{Feature Patterns Before ASSA Module}
    \end{subfigure}%

    \begin{subfigure}{6in}
    \centering
        \includegraphics[height=28mm]{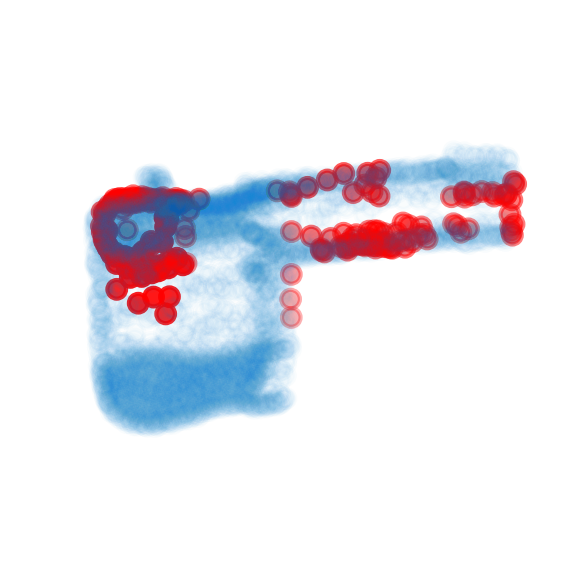}
        \includegraphics[height=28mm]{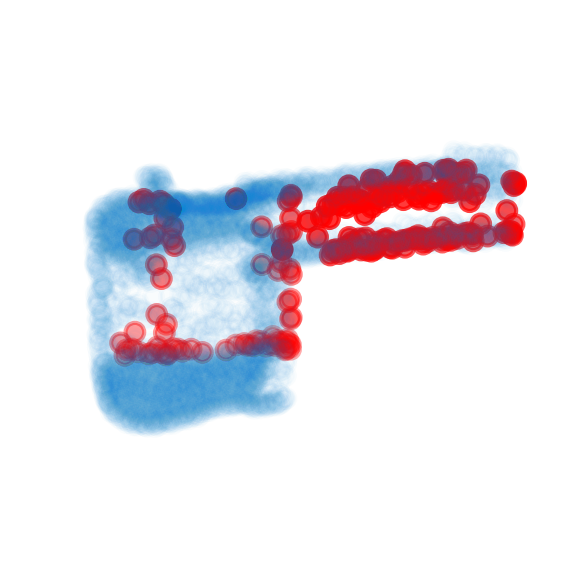}
        \includegraphics[height=28mm]{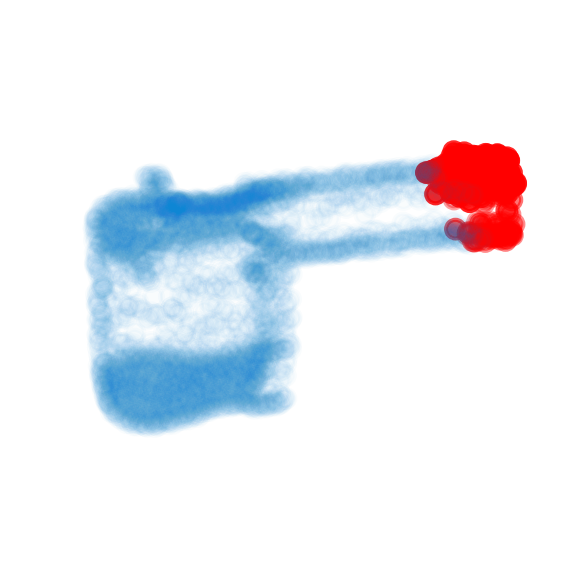}
        \includegraphics[height=28mm]{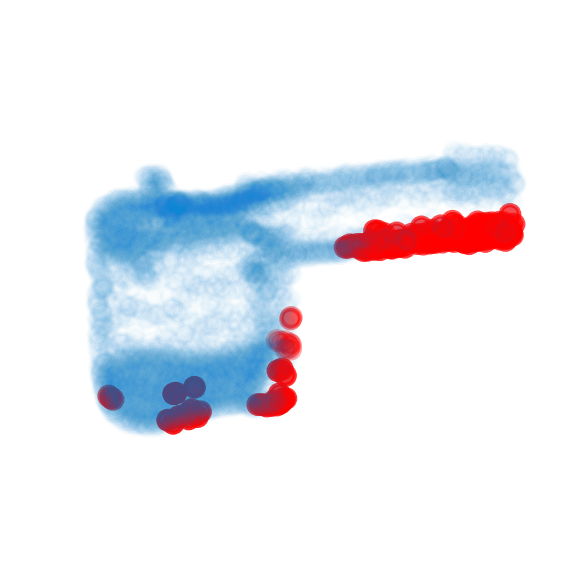}
        \includegraphics[height=28mm]{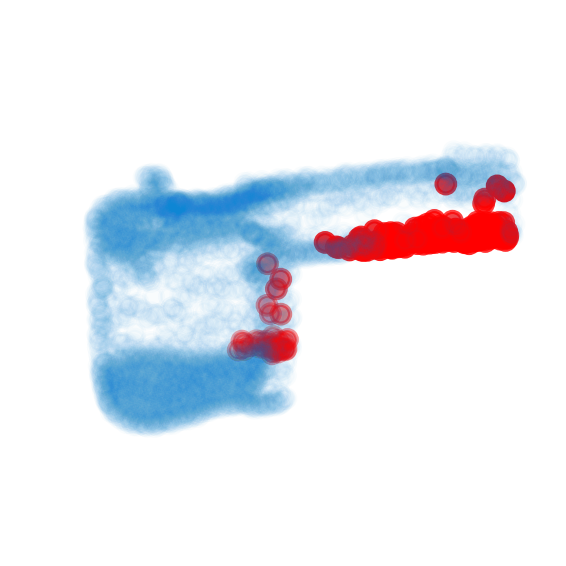}
    \end{subfigure}%
    
    \begin{subfigure}{6in}
    \centering
        \includegraphics[height=28mm]{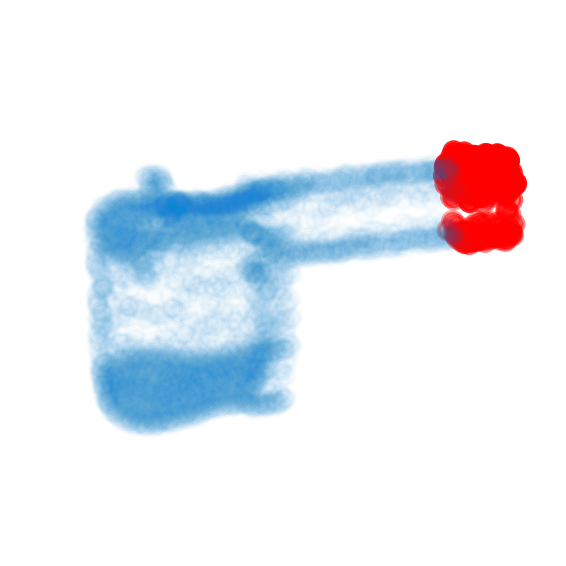}
        \includegraphics[height=28mm]{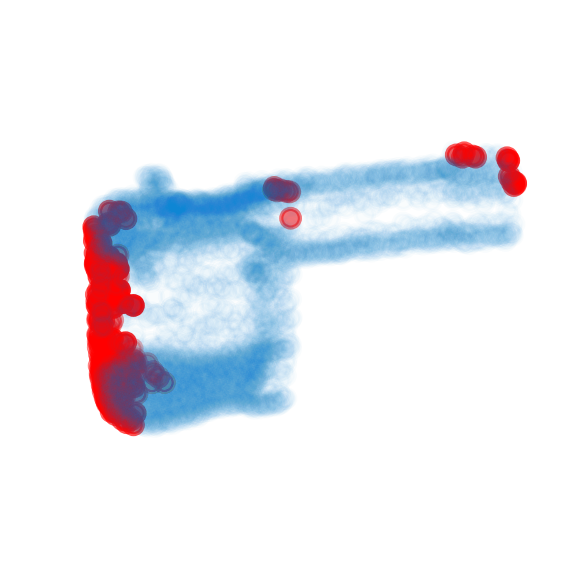}
        \includegraphics[height=28mm]{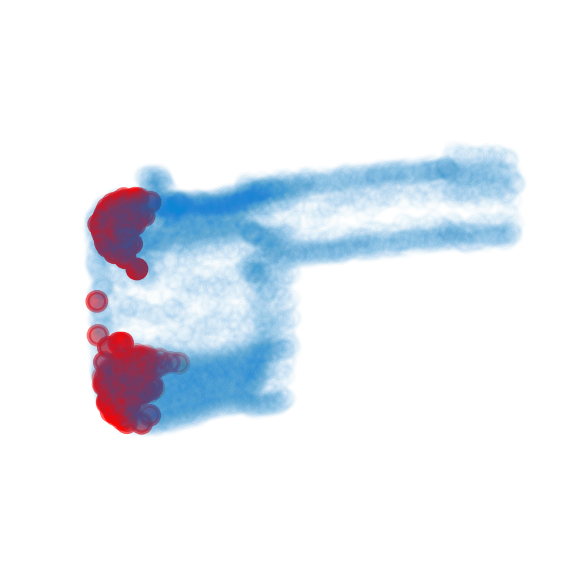}
        \includegraphics[height=28mm]{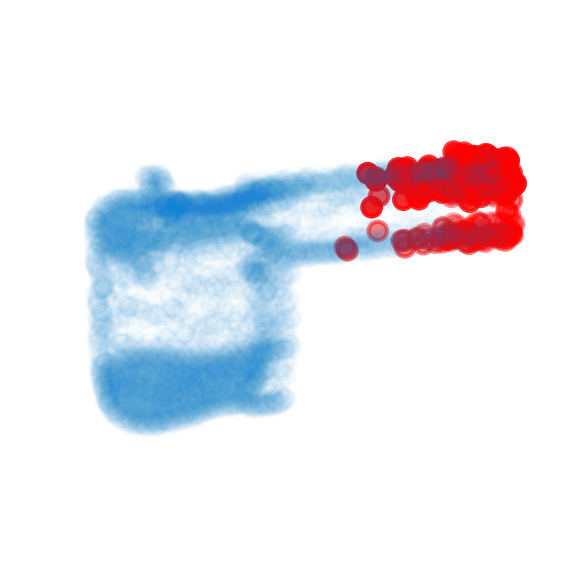}
        \includegraphics[height=28mm]{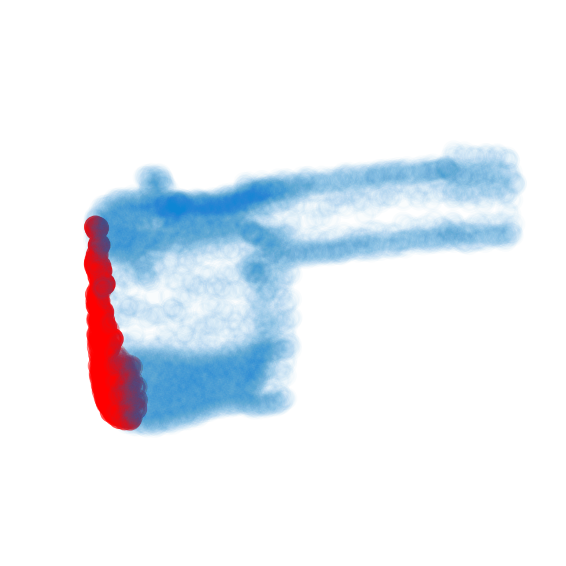}
    \end{subfigure}%
    
    \begin{subfigure}{6in}
    \centering
        \includegraphics[height=28mm]{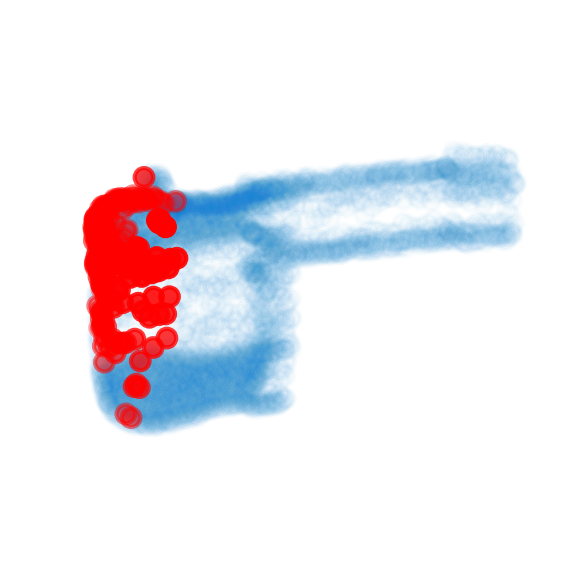}
        \includegraphics[height=28mm]{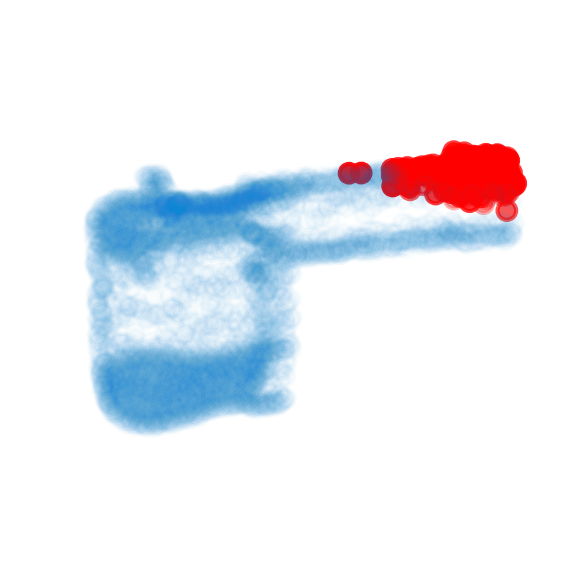}
        \includegraphics[height=28mm]{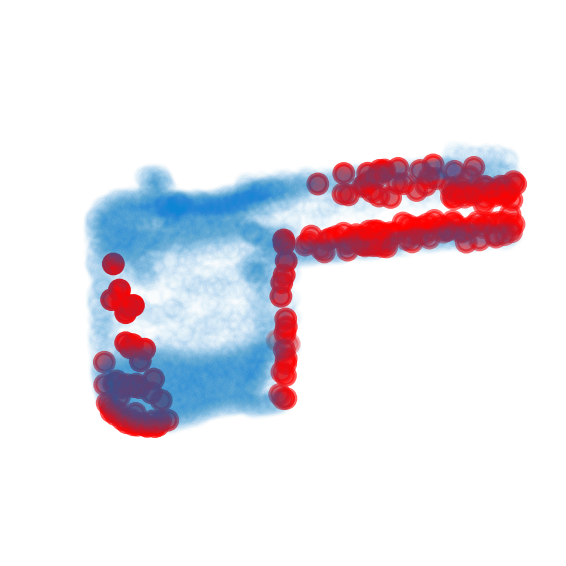}
        \includegraphics[height=28mm]{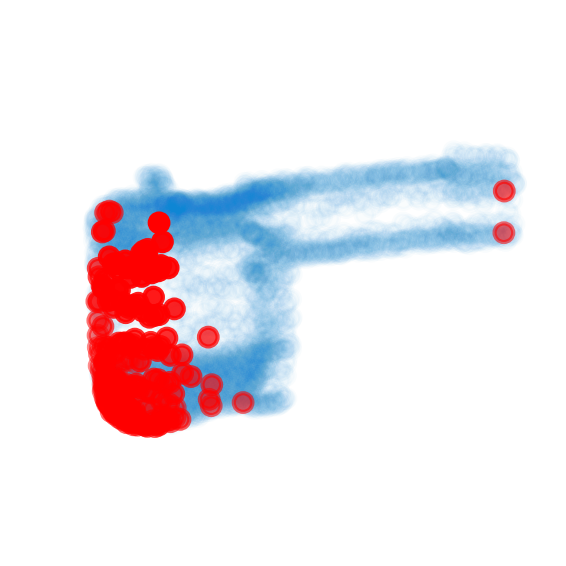}
        \includegraphics[height=28mm]{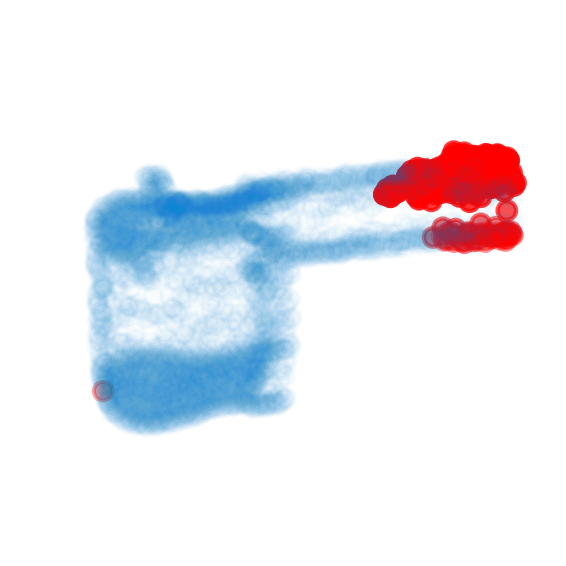}
        \caption{Feature Patterns After ASSA Module}
        
    \end{subfigure}%

\caption{Guitar feature patterns visualization}
\label{fig:feature_pattern5}
\end{figure}

\begin{figure}[!ht]

    \begin{subfigure}{6in}
    \centering
        \includegraphics[height=28mm]{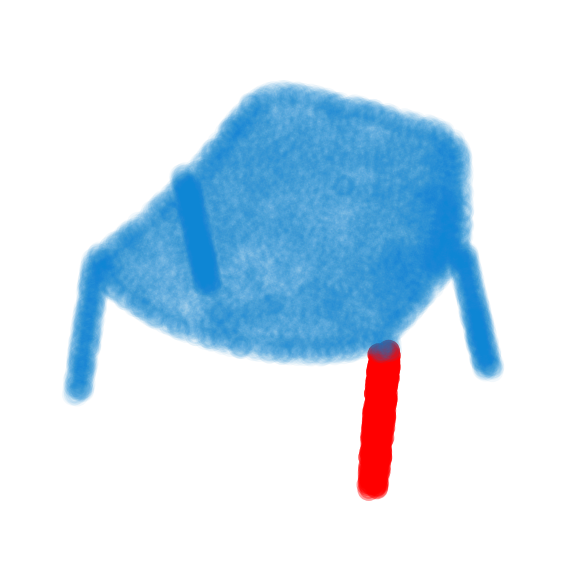}
        \includegraphics[height=28mm]{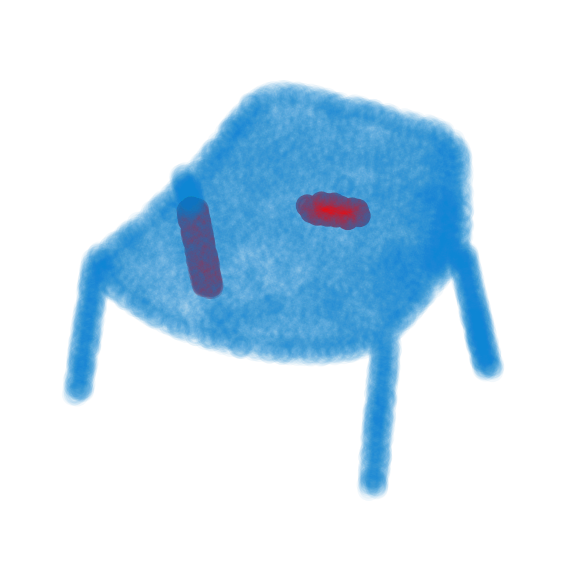}
        \includegraphics[height=28mm]{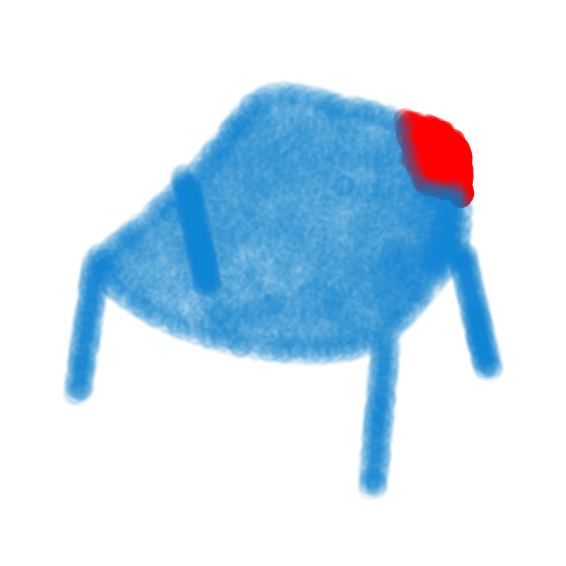}
        \includegraphics[height=28mm]{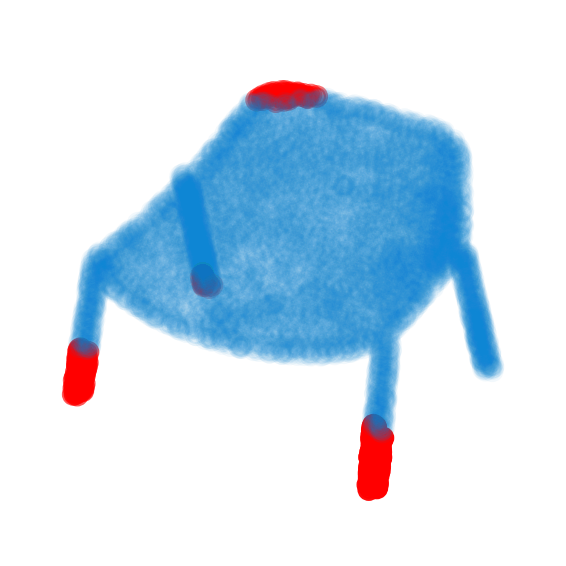}
        \includegraphics[height=28mm]{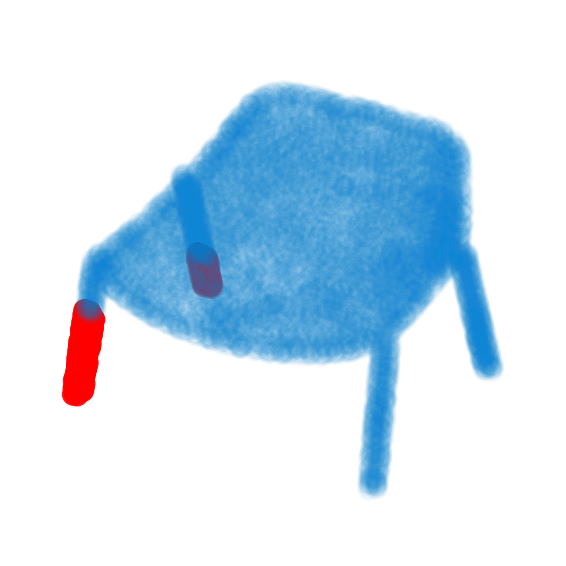}
        \caption{Feature Patterns Before ASSA Module}
    \end{subfigure}%

    \begin{subfigure}{6in}
    \centering
        \includegraphics[height=28mm]{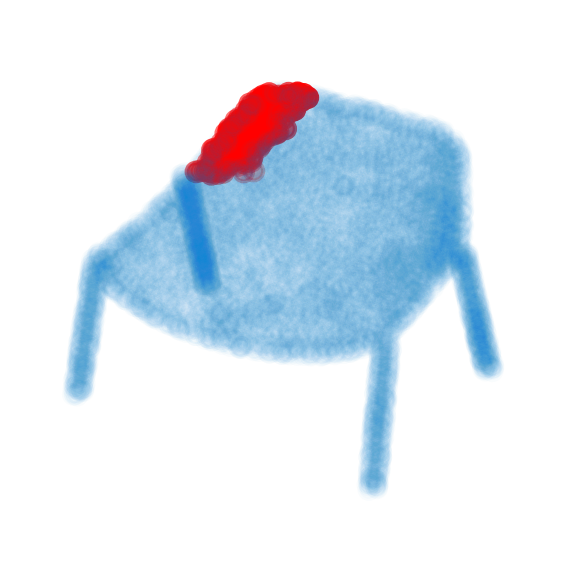}
        \includegraphics[height=28mm]{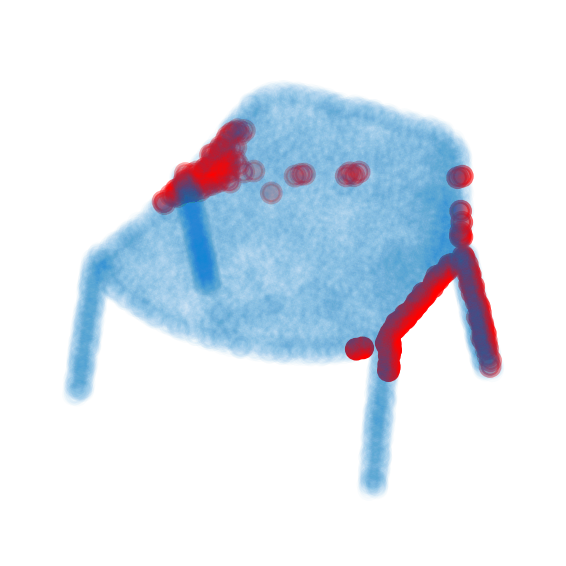}
        \includegraphics[height=28mm]{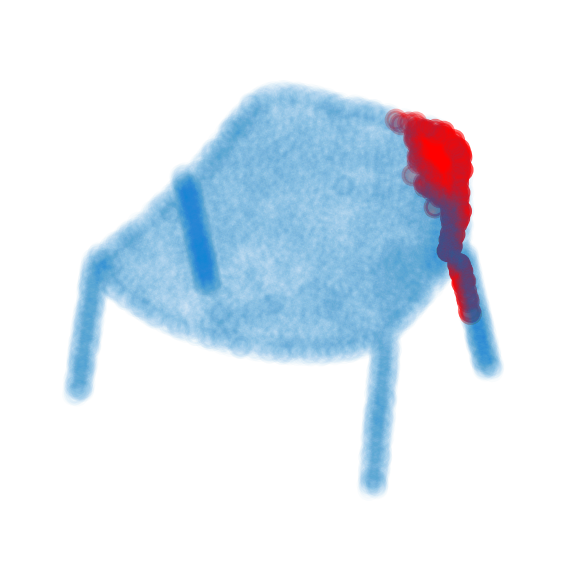}
        \includegraphics[height=28mm]{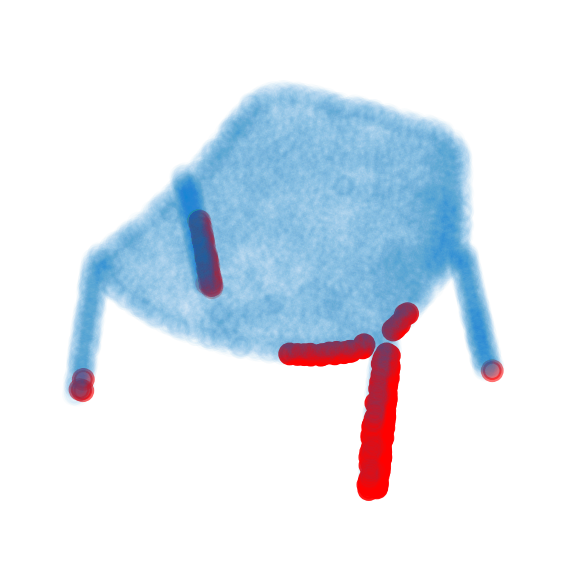}
        \includegraphics[height=28mm]{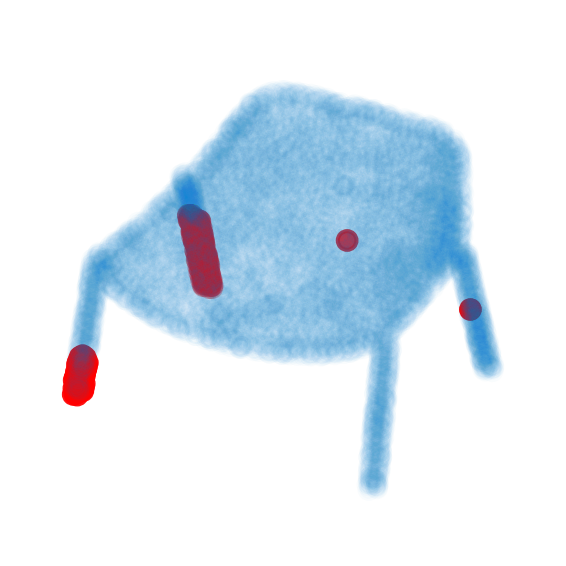}
    \end{subfigure}%
    
    \begin{subfigure}{6in}
    \centering
        \includegraphics[height=28mm]{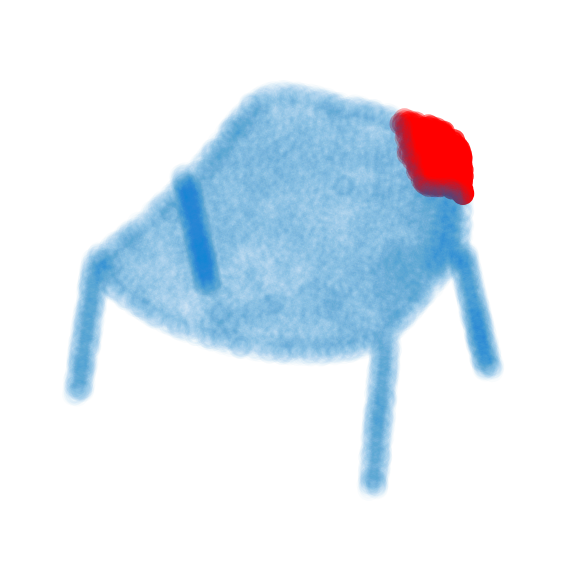}
        \includegraphics[height=28mm]{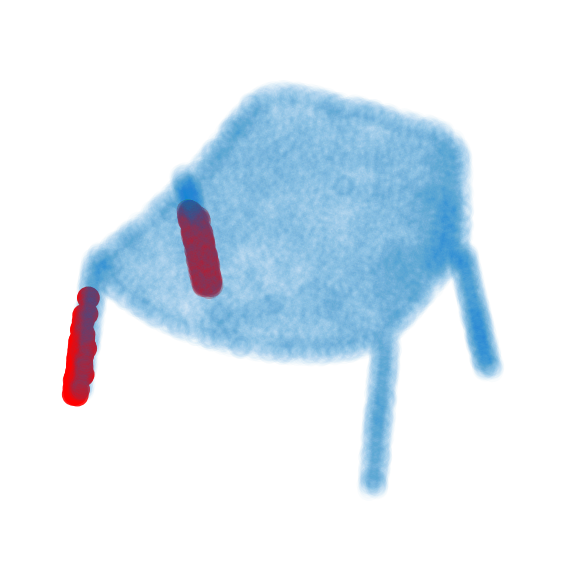}
        \includegraphics[height=28mm]{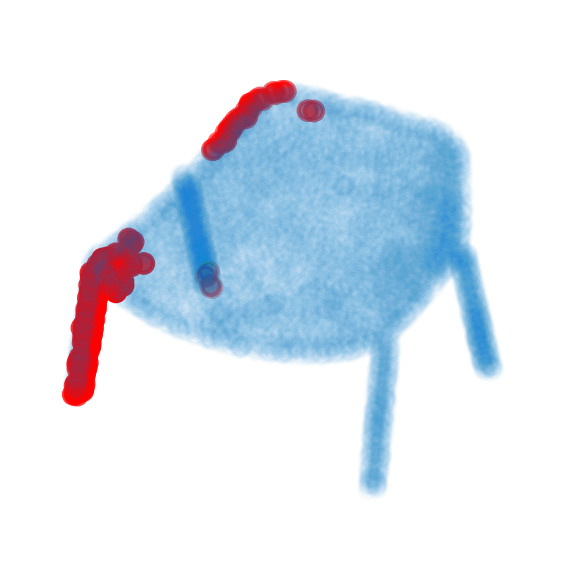}
        \includegraphics[height=28mm]{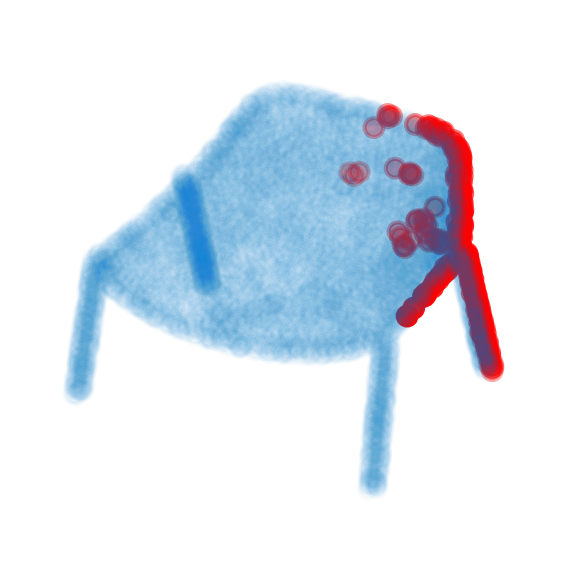}
        \includegraphics[height=28mm]{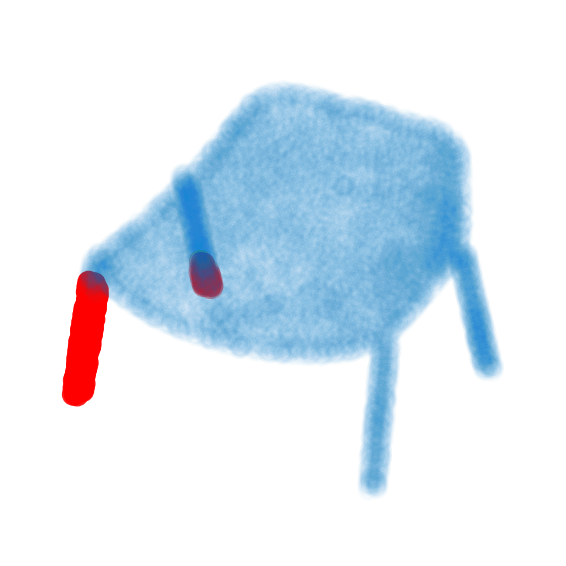}
    \end{subfigure}%
    
    \begin{subfigure}{6in}
    \centering
        \includegraphics[height=28mm]{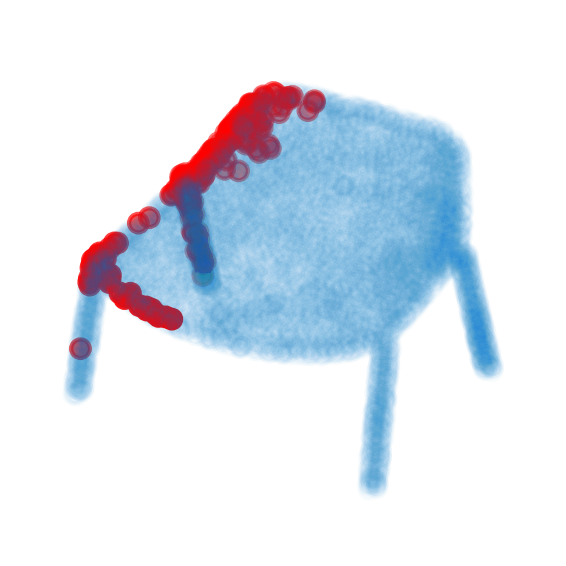}
        \includegraphics[height=28mm]{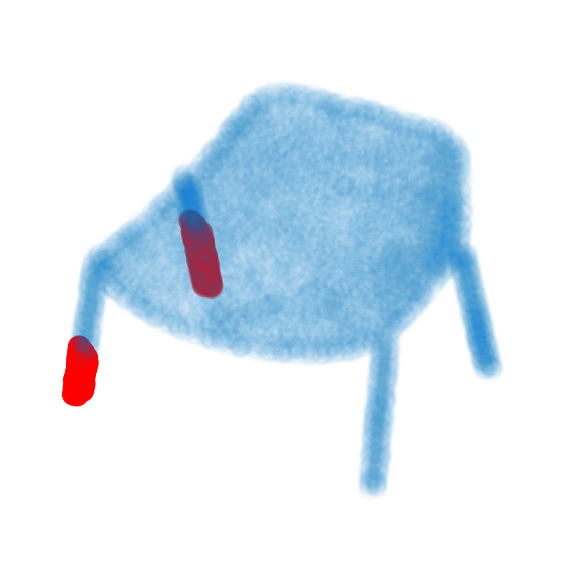}
        \includegraphics[height=28mm]{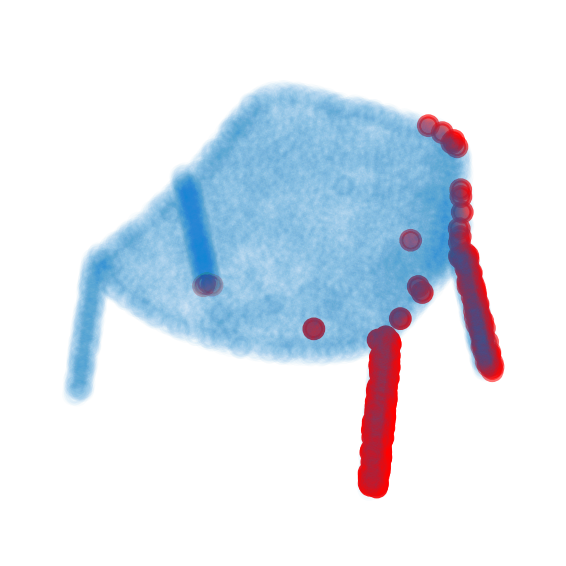}
        \includegraphics[height=28mm]{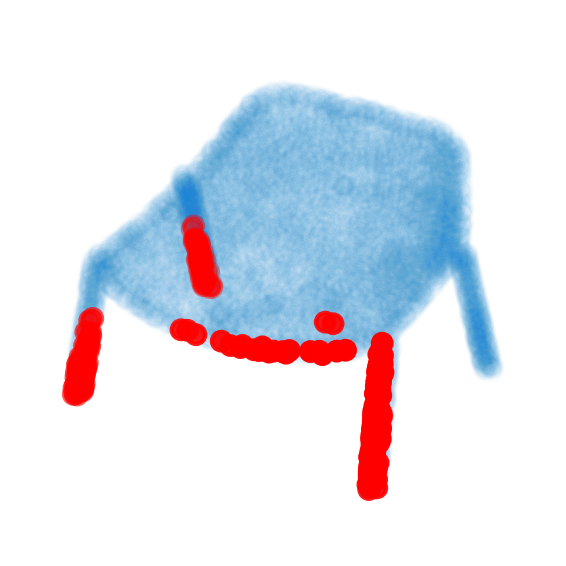}
        \includegraphics[height=28mm]{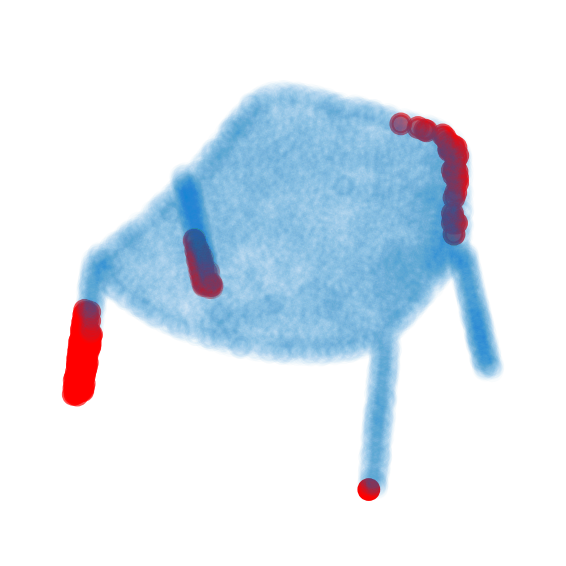}
        \caption{Feature Patterns After ASSA Module}
        
    \end{subfigure}%

\caption{Chair feature patterns visualization}
\label{fig:feature_pattern6}
\end{figure}

\begin{figure}[!ht]

    \begin{subfigure}{6in}
    \centering
        \includegraphics[height=28mm]{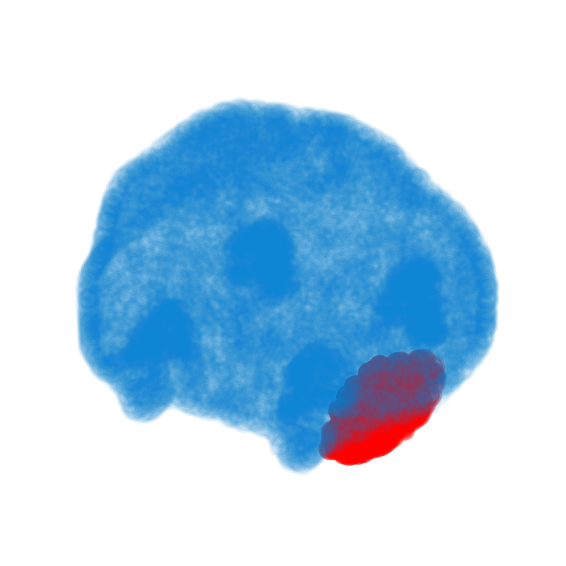}
        \includegraphics[height=28mm]{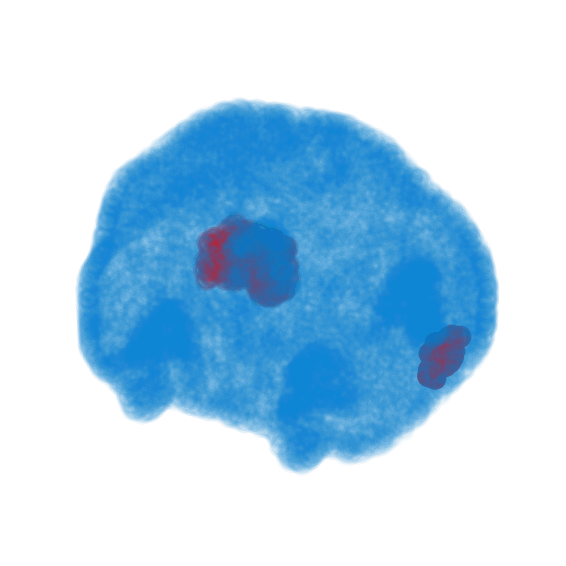}
        \includegraphics[height=28mm]{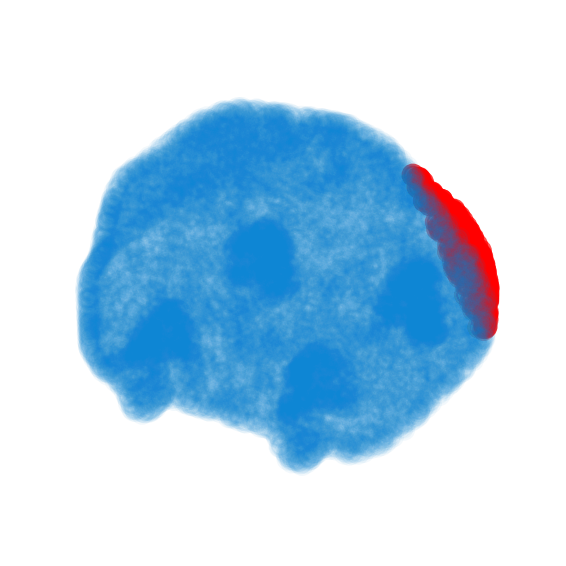}
        \includegraphics[height=28mm]{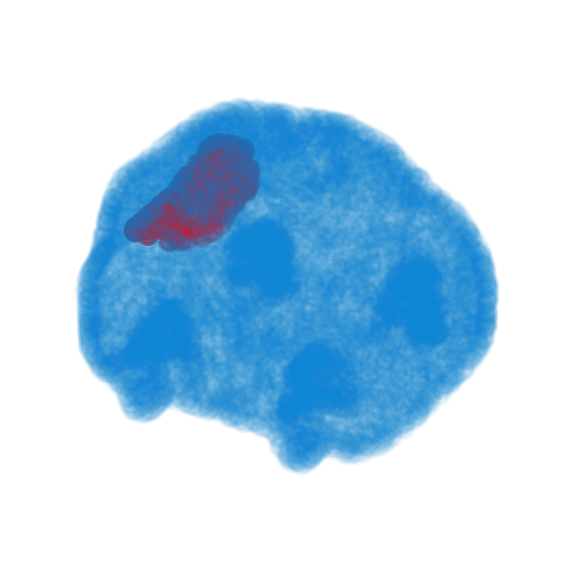}
        \includegraphics[height=28mm]{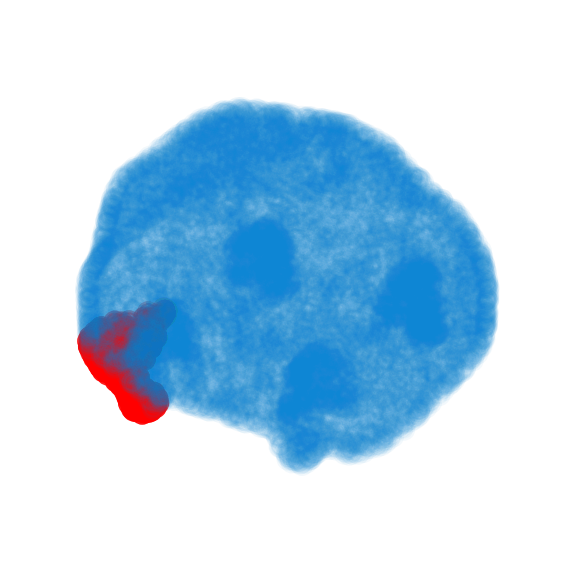}
        \caption{Feature Patterns Before ASSA Module}
    \end{subfigure}%

    \begin{subfigure}{6in}
    \centering
        \includegraphics[height=28mm]{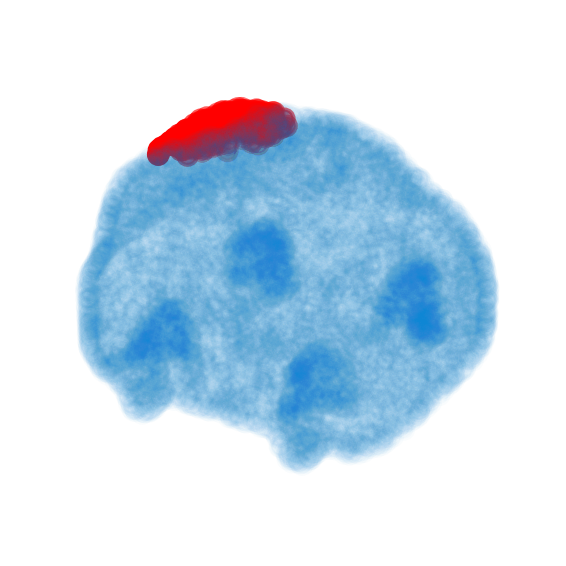}
        \includegraphics[height=28mm]{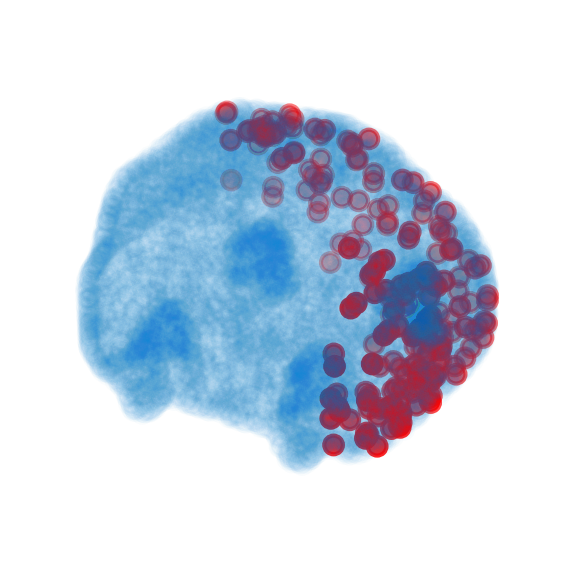}
        \includegraphics[height=28mm]{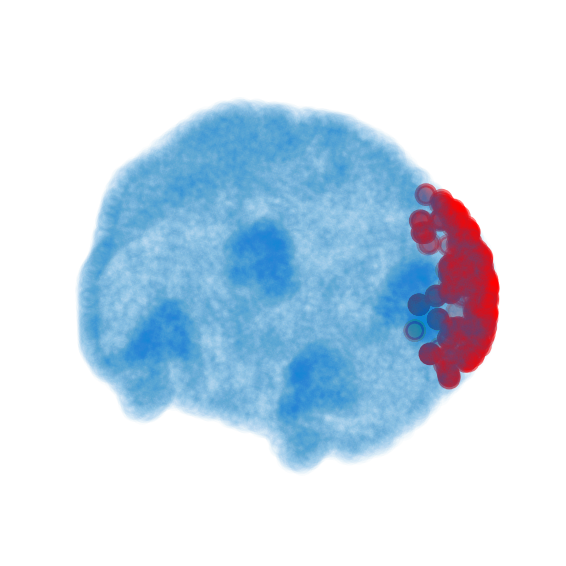}
        \includegraphics[height=28mm]{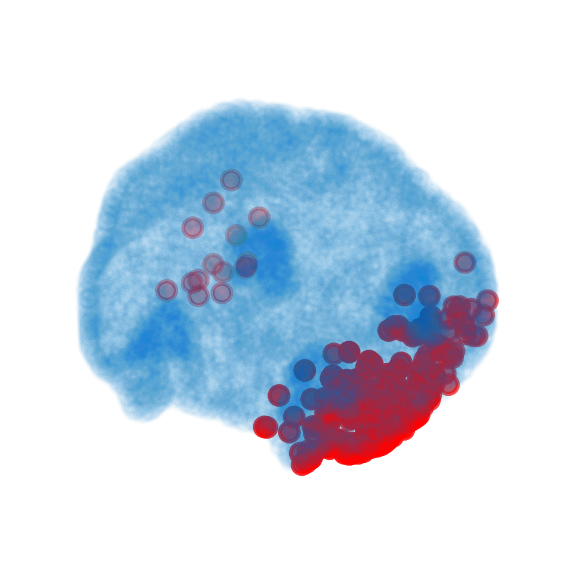}
        \includegraphics[height=28mm]{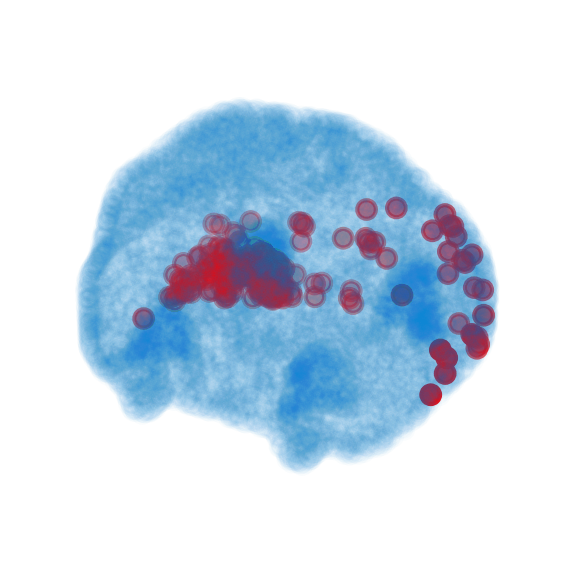}
    \end{subfigure}%
    
    \begin{subfigure}{6in}
    \centering
        \includegraphics[height=28mm]{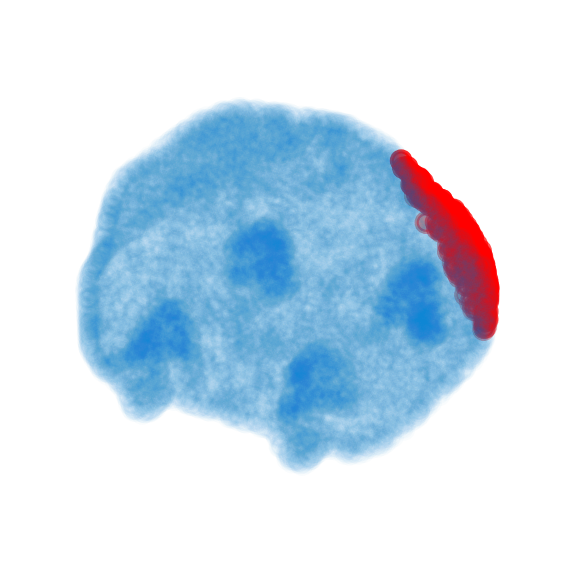}
        \includegraphics[height=28mm]{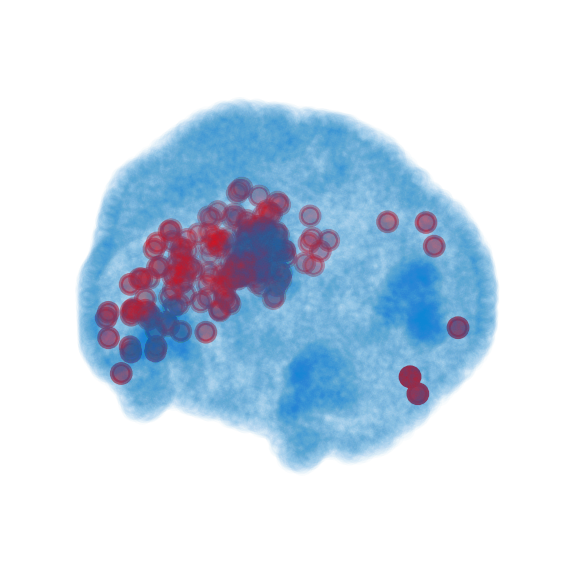}
        \includegraphics[height=28mm]{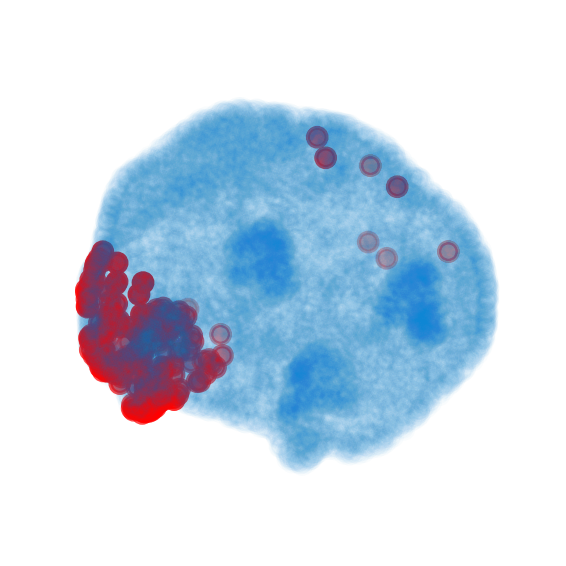}
        \includegraphics[height=28mm]{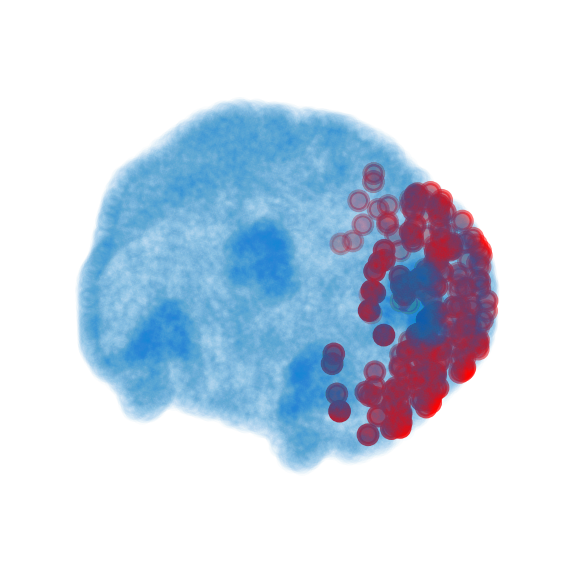}
        \includegraphics[height=28mm]{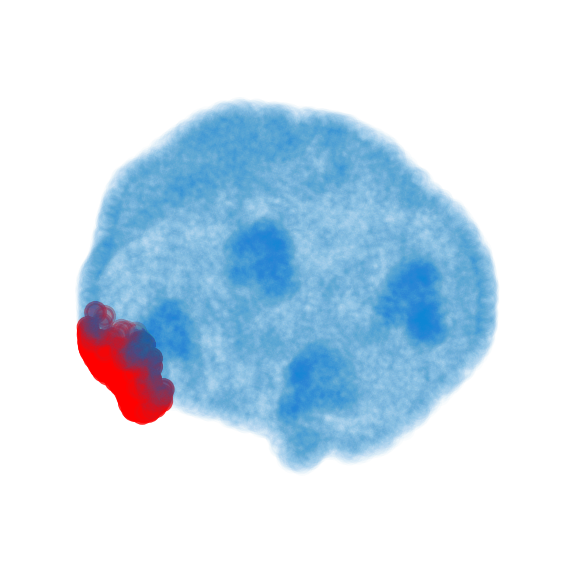}
    \end{subfigure}%
    
    \begin{subfigure}{6in}
    \centering
        \includegraphics[height=28mm]{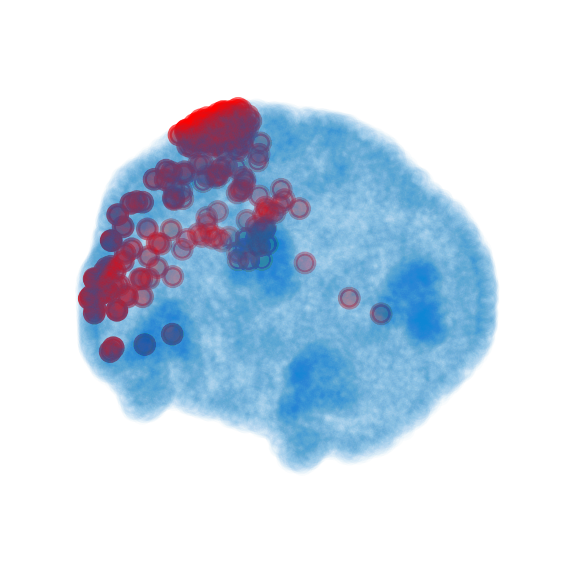}
        \includegraphics[height=28mm]{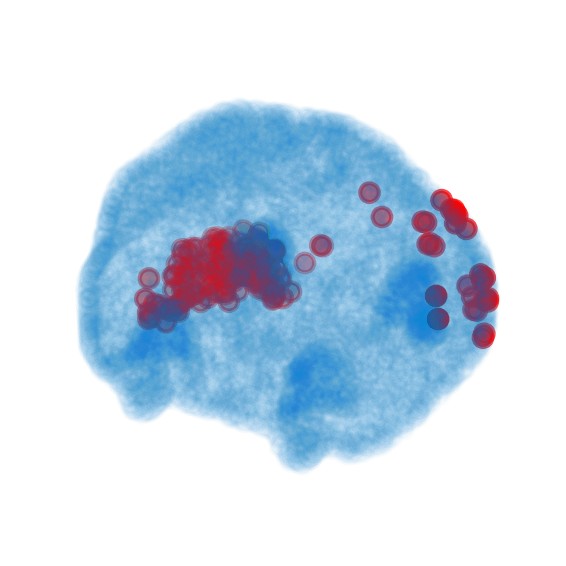}
        \includegraphics[height=28mm]{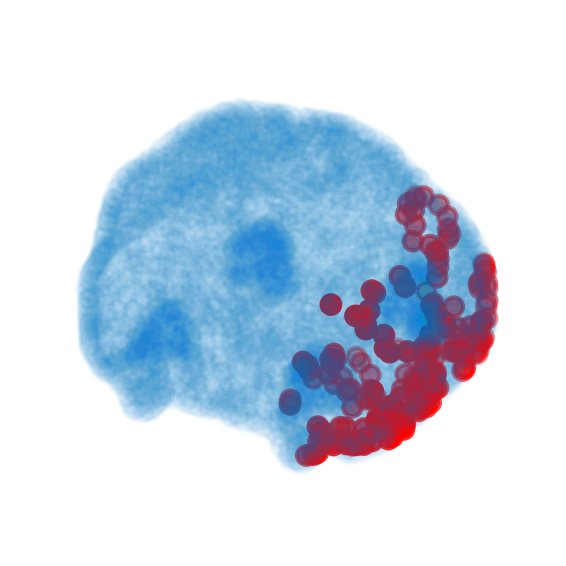}
        \includegraphics[height=28mm]{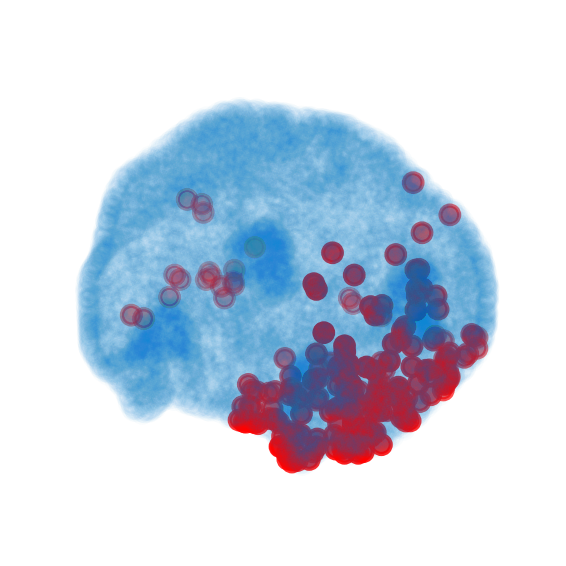}
        \includegraphics[height=28mm]{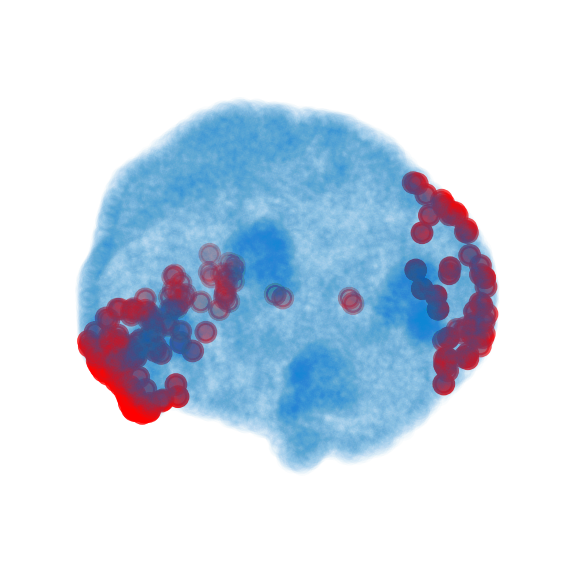}
        \caption{Feature Patterns After ASSA Module}
        
    \end{subfigure}%

\caption{Car feature patterns visualization}
\label{fig:feature_pattern8}
\end{figure}
